# Supplementary material for: Robust Graph Representation Learning via Predictive Coding
Source: arXiv:2212.04656 source file (2022-12-09)
Supplement: Supplementary file 2 [file Appendices.tex]

\appendix

\section{Details on evaluation metrics}

In this section, we explain the metrics used in the main body of this work in more detail. We employ scalar quantification metrics, such as expected calibration error (ECE) and maximum calibration error, together with visual tools, such as reliability diagrams and confidence distribution histograms \citep{guo2017calibration} and classification margin diagrams \citep{dai2018adversarial} to evaluate model calibration.

The term `confidence calibration` is used to describe the ability of a model to produce probability estimations that are accurate reflections of the correct likelihood an event, which is imperative especially in real-world applications. Considering a $K$-class classification task, let  $X \in \mathcal{X}$ and $Y \in \mathcal{Y}=\{1, \ldots, K\}$ be input and true ground truth label random variables, respectively. Let $\hat{Y}$ denote a class prediction and $\hat{P}$ be its associated confidence, i.e. probability of correctness. We would like the confidence estimate $\hat{P}$ to be calibrated, which intuitively means that $\hat{P}$ represents a true probability. The perfect calibration can be described as follows:
\begin{equation}
\label{eqn:calibration}
    \mathbb{P}(\hat{Y}=Y \mid \hat{P}=p)=p, \quad \forall p \in[0,1]
\end{equation}
\textbf{ECE} captures the notion of average miscalibration in a single number, and can be obtained by the expected difference between  accuracy and confiedence of the model: $
\underset{\hat{P}}{\mathbb{E}}[|\mathbb{P}(\hat{Y}=Y \mid \hat{P}=p)-p|]
$

\textbf{MCE} is much crucial in safety-, security-critical settings, as it quantifies worst-case expected miscalibration: $
\max _{p \in[0,1]}|\mathbb{P}(\hat{Y}=Y \mid \hat{P}=p)-p| .
$

\textbf{Reliability diagrams} are visual representation tools for model calibration as equation~\ref{eqn:calibration} is intractable because  $\hat{P}$ is a continuous random variable. They characterise the average accuracy level inside a points that feels into a given confidence level bin (see \cite{} for more details on formulation of the the above metrics).

\textbf{Classification margin} is simply the difference between the model output probability of the ground truth class and the model probability of the predicted most-likely class, i.e.,the probability of the best second class. Thus, this metric is between $-1$ and $1$, where values close to $-1$ indicate that a model is overconfident in wrong predictions and values closer to $1$ indicate that the model is confidence in its correct prediction. In our reported class margin diagrams,  we average these values over many samples and repeated trials with different random seeds to draw box-plot diagrams of our results.

\section{Reproducibility}

We use standard splits on all datasets. We report the average results of 5 runs on different seeds; the hyper-parameters are selected using the validation set. Following the results from original papers on baseline models, we evaluate our model on 2 GNN layers. The models are trained for 300 epochs on citation graphs and 50 epochs on PPI. We also use Adam optimiser. The reported results on calibration analysis were performed on initial learning rate of 0.001 for both GCN and GPCN as it provided best performances for both models. For adversarial attacks, we set initial learning rate to 0.01 and epochs to 200 to compare our results to other works. For general performance experiment, we use grid search for hyper-parameters as described in Table~\ref{tab:hyperpar}. Inductive tasks were trained using GCN version of GraphSage \citep{hamilton2017inductive} with neighborhood sample size of 25 and 10 for first and second GNN layer, respectively (see \cite{hamilton2017inductive} for more details).

Our experiments are performed using Pytorch Geometric library \cite{fey2019fast}. In order to do an extensive experiment, we build on GraphGym \cite{you2020design}, a research platform for designing and evaluating GNNs, and we seamlessly integrate it with predictive coding learning algorithm. In addition, we employ another Pytorch library for adversarial attacks and defenses known as Deeprobust \cite{li2020deeprobust} for various type of adversarial attacks we perform on graphs.

\subsection{Datasets}
\begin{table}[H]
    \caption{An overview of the data sets used in our experiments }\label{tab:datasets}
    \begin{adjustbox}{max width=\textwidth}
    \begin{tabular}{*{7}{|c}|}\hline
    %   • &\multicolumn{8}{c|}{West Hebrides} \\
    %  \hline
    %  • & \multicolumn{2}{c|}{$H_{s}$} &\multicolumn{2}{c|}{$T_{p}$} &\multicolumn{2}{c|}{$T_{z}$} & \multicolumn{2}{c|}{Dir} \\
    %  \hline
       & Cora & Citeseer &  Pubmed & PPI &  Reddit \\
    %  \hline
    %  Task & • & • & • & • & • & • & •   \\
     \hline
     Type & Citation & Citation & Citation & Protein interaction & Communities  \\
     \hline
     \#Nodes & 2708 & 3327 & 19717 (1 graph) & 56944 (24 graphs) & 232965 (1 graph) \\
     \hline
     \#Edges  & 5429 & 4732 & 44338 & 818716 & 114615892   \\
     \hline
     \#Features/Nodes & 1433 & 3703 & 500 & 50 & 602   \\
     \hline
     \#Classes & 7 & 6 & 3 & 121(multilabel) & 41   \\
     \hline
     \#Training Nodes & 140 & 120 & 60 & 44906(20 graphs) & 153431    \\
     \hline
     \#Validation Nodes & 500 & 500 & 500 & 6513 (2 graphs) & 23831  \\
     \hline
     \#Testing Nodes  & 1000 & 1000 & 1000 & 5524 (2 graphs) & 55703   \\
     \hline
 \end{tabular}
 \end{adjustbox}
\end{table}

\begin{table}[H]
  \centering
  \begin{tabular}{|c|c|c|}
    \hline
    Parameter Type & Grid \\
    \hline
    values nodes update rate & $0.05, 0.1, 0.5, 1.0$  \\
    Weight update learning rate & $1e-2$,$1e-3$,$1e-4$,$1e-5$ \\
    Number of GNN Layer & $2, 4$ \\
   Inference steps,T, & 12, 32, 50, 100\\
    PC synaptic weight update rate &  at the end of ,T, inference steps, and at every inference step\\
    aggregation functions  &  sum, add, max\\
    Graphsage sampling & 10, 25 for first and second GNN layer respectively\\
    \hline
  \end{tabular}
  \caption{Hyper-Parameter Search}\label{tab:hyperpar}
\end{table}

\section{Calibration Analysis: Confidence in Prediction} 
As deep networks tend to be overconfident even if they are wrong, we compared the confidence distribution of GPCNs with GCNs in Figure~\ref{fig:conf_distribution_cora},~\ref{fig:conf_distribution_citeseer}, and \ref{fig:conf_distribution}, where confidence is the maximum of the softmax of the model output. The result in this section correspond to the reported results in the body of the paper on calibration analysis in Section~\ref{sec:cal_analysis}. Both model are run for 300 epochs using the same parameters (i.e., learning rate on weights equal to 0.001) and we select the best model based on validation set for GCN. For GPCN, we select the best model based on best accuracy on validation set as well as lowest energy on training set as the energy minimization can be interpreted as likelihood maximisation. We consider energy while selecting the best model for evaluation because we discovered a high correlation between energy and robustness as we will demonstrate in the following section (see Figure~\ref{fig:energy_calibration}). Interestingly, the results on prediction distribution on provide another dimension to communicate the same results we witness in Section~\ref{sec:cal_analysis} using reliability diagrams. We see that on the prediction distribution on Cora dataset in Figure~\ref{fig:conf_distribution}, GPCNs are relatively less confident in their predictions, while GCN model is overly confident. Figure~\ref{fig:conf_distribution_citeseer} on Citeseer dataset similarly here shows that most prediction confidence of GCN model are less than 0.5, showing that GCN models are overly under-confident as we saw in the body of the paper. GPCNs models on the other hand provide a well behaved prediction confidence distribution on Citeseer. demonstrate that either GCN either is under-confident despite high performance accuracy or over-confident in the manner that is disproportional to its performance accuracy.

\begin{figure}[H]
    \centering
    {{\includegraphics[width=6.5cm]{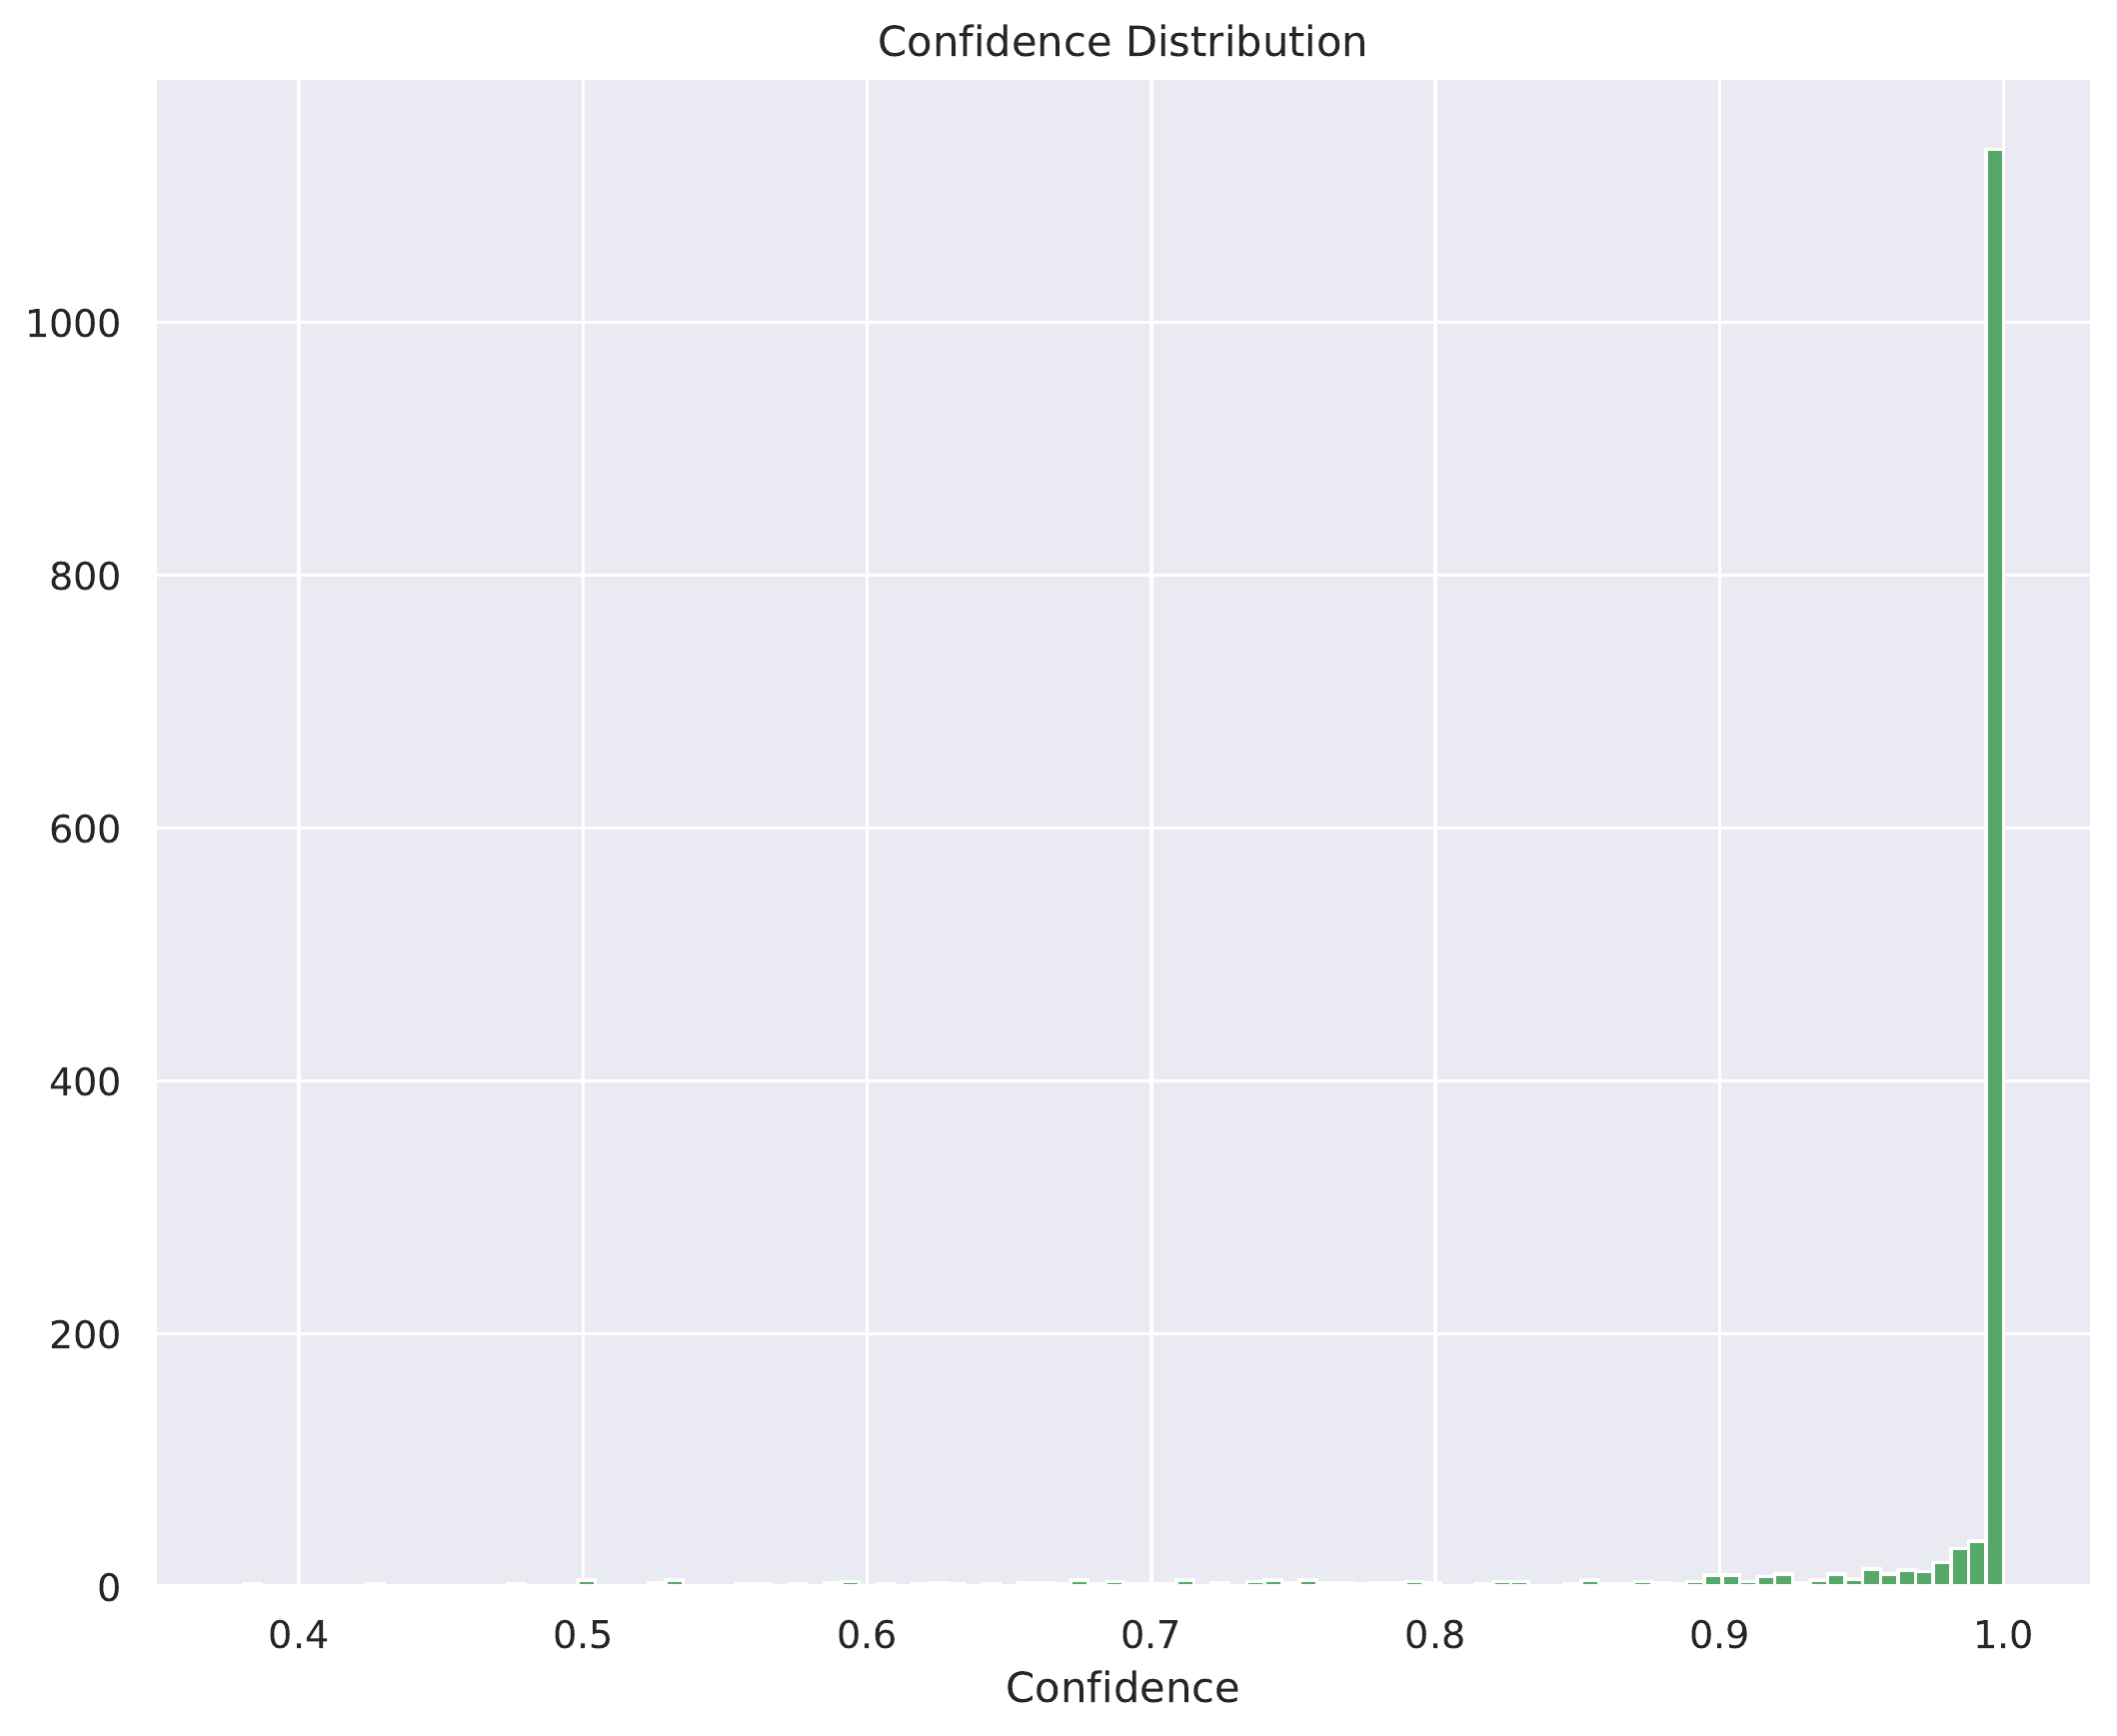} }}%
    \qquad
    {{\includegraphics[width=6.5cm]{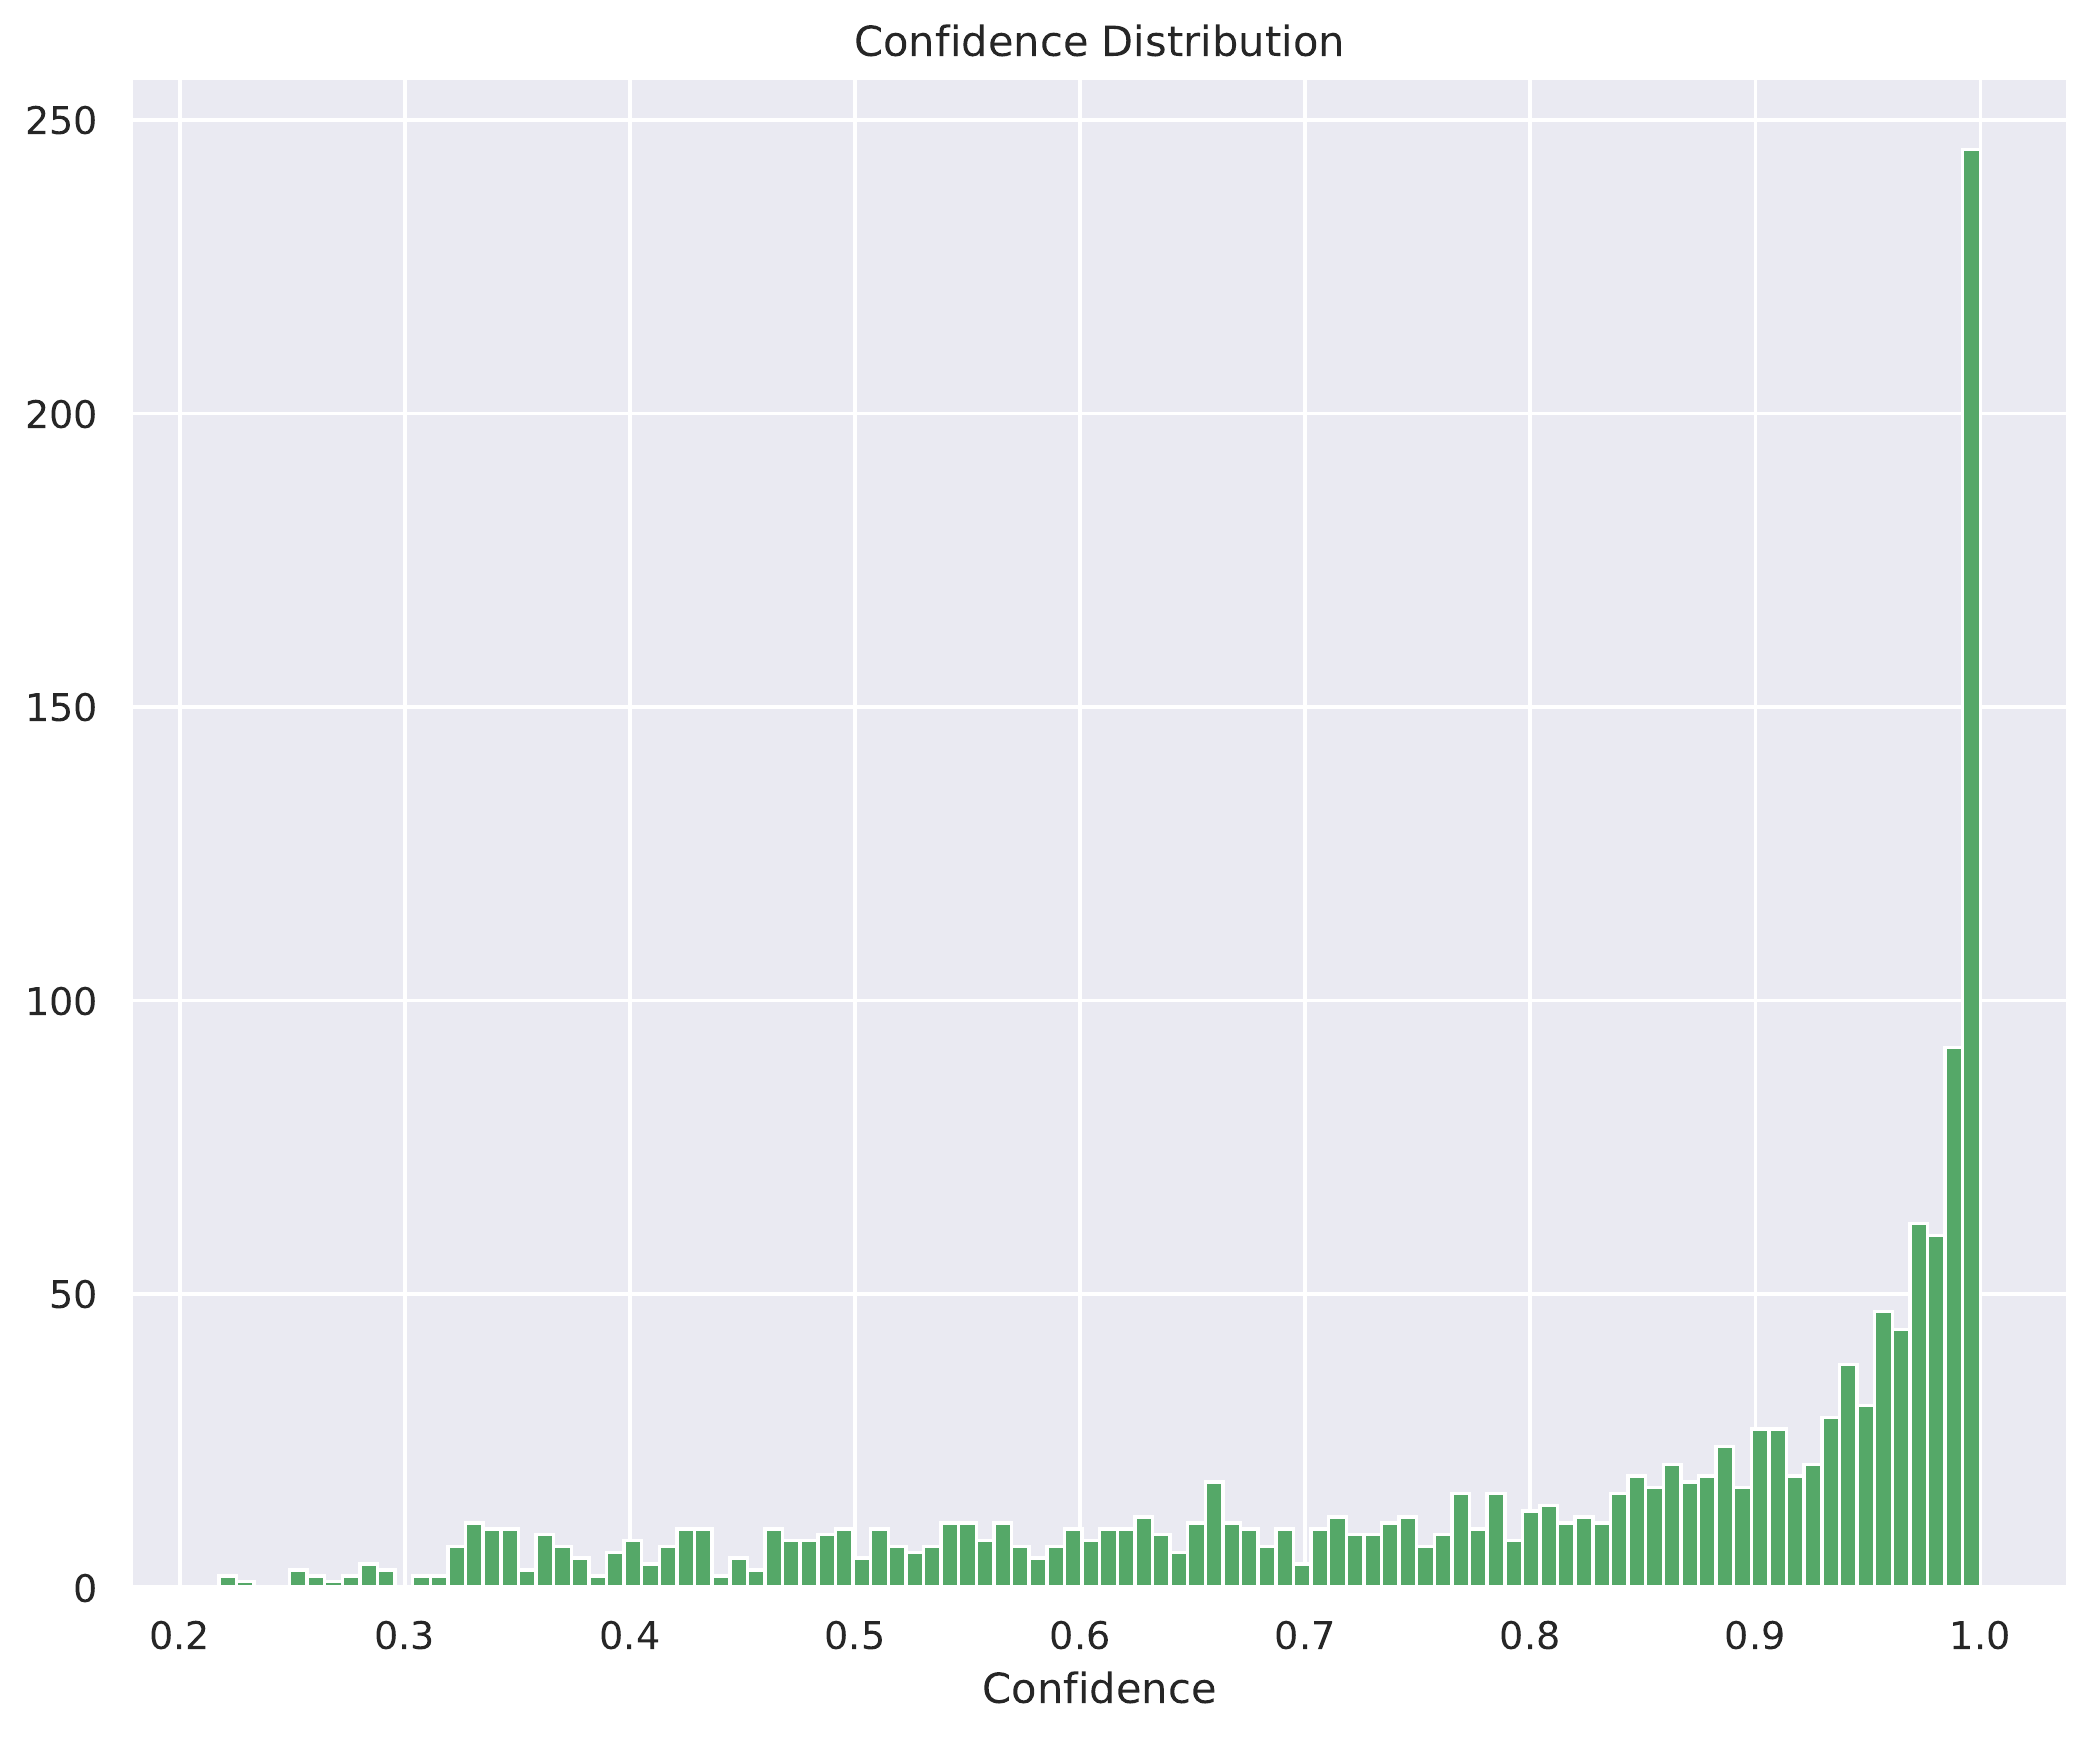} }}%
    \caption{Histogram of prediction confidence distribution on Cora dataset. The x-axis indicates the confidence of the model on the samples, and y-axis is the count on a normal scale of data points that fall into a given confidence bin. Left: GCN. Right: GPCN.}%
    \label{fig:conf_distribution_cora}%
\end{figure}

\begin{figure}[H]
    \centering
    {{\includegraphics[width=6.5cm]{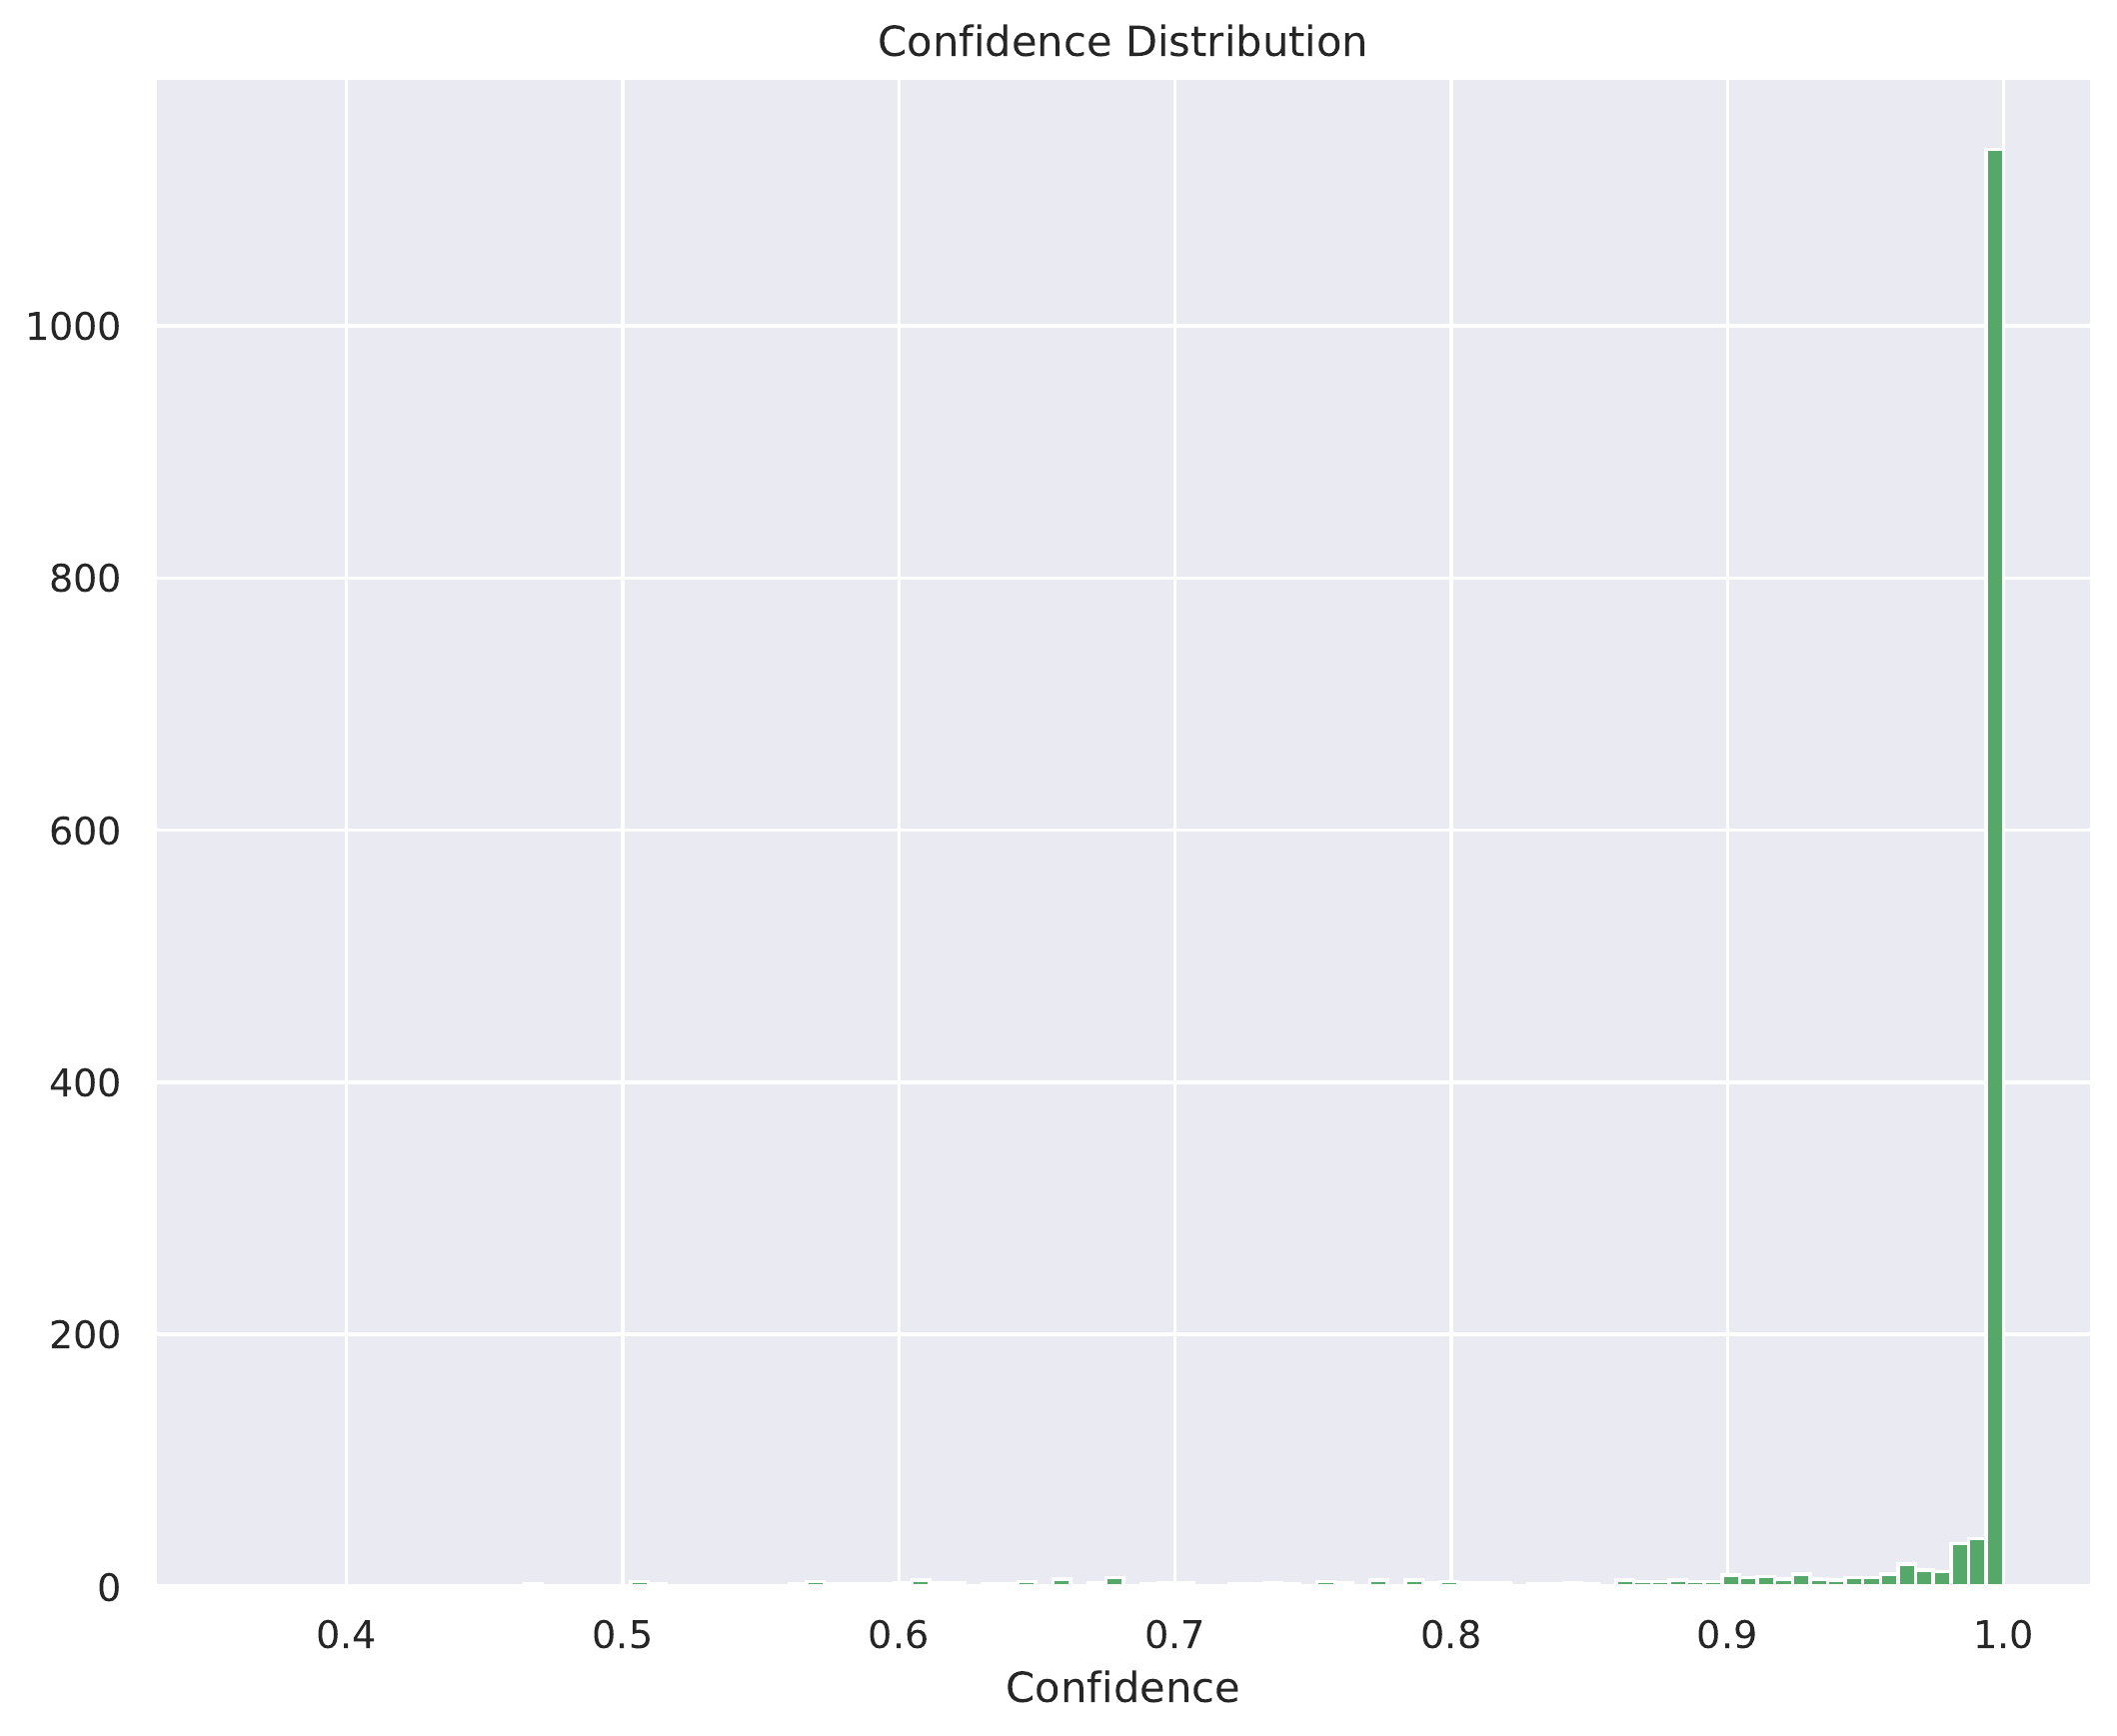} }}%
    \qquad
    {{\includegraphics[width=6.5cm]{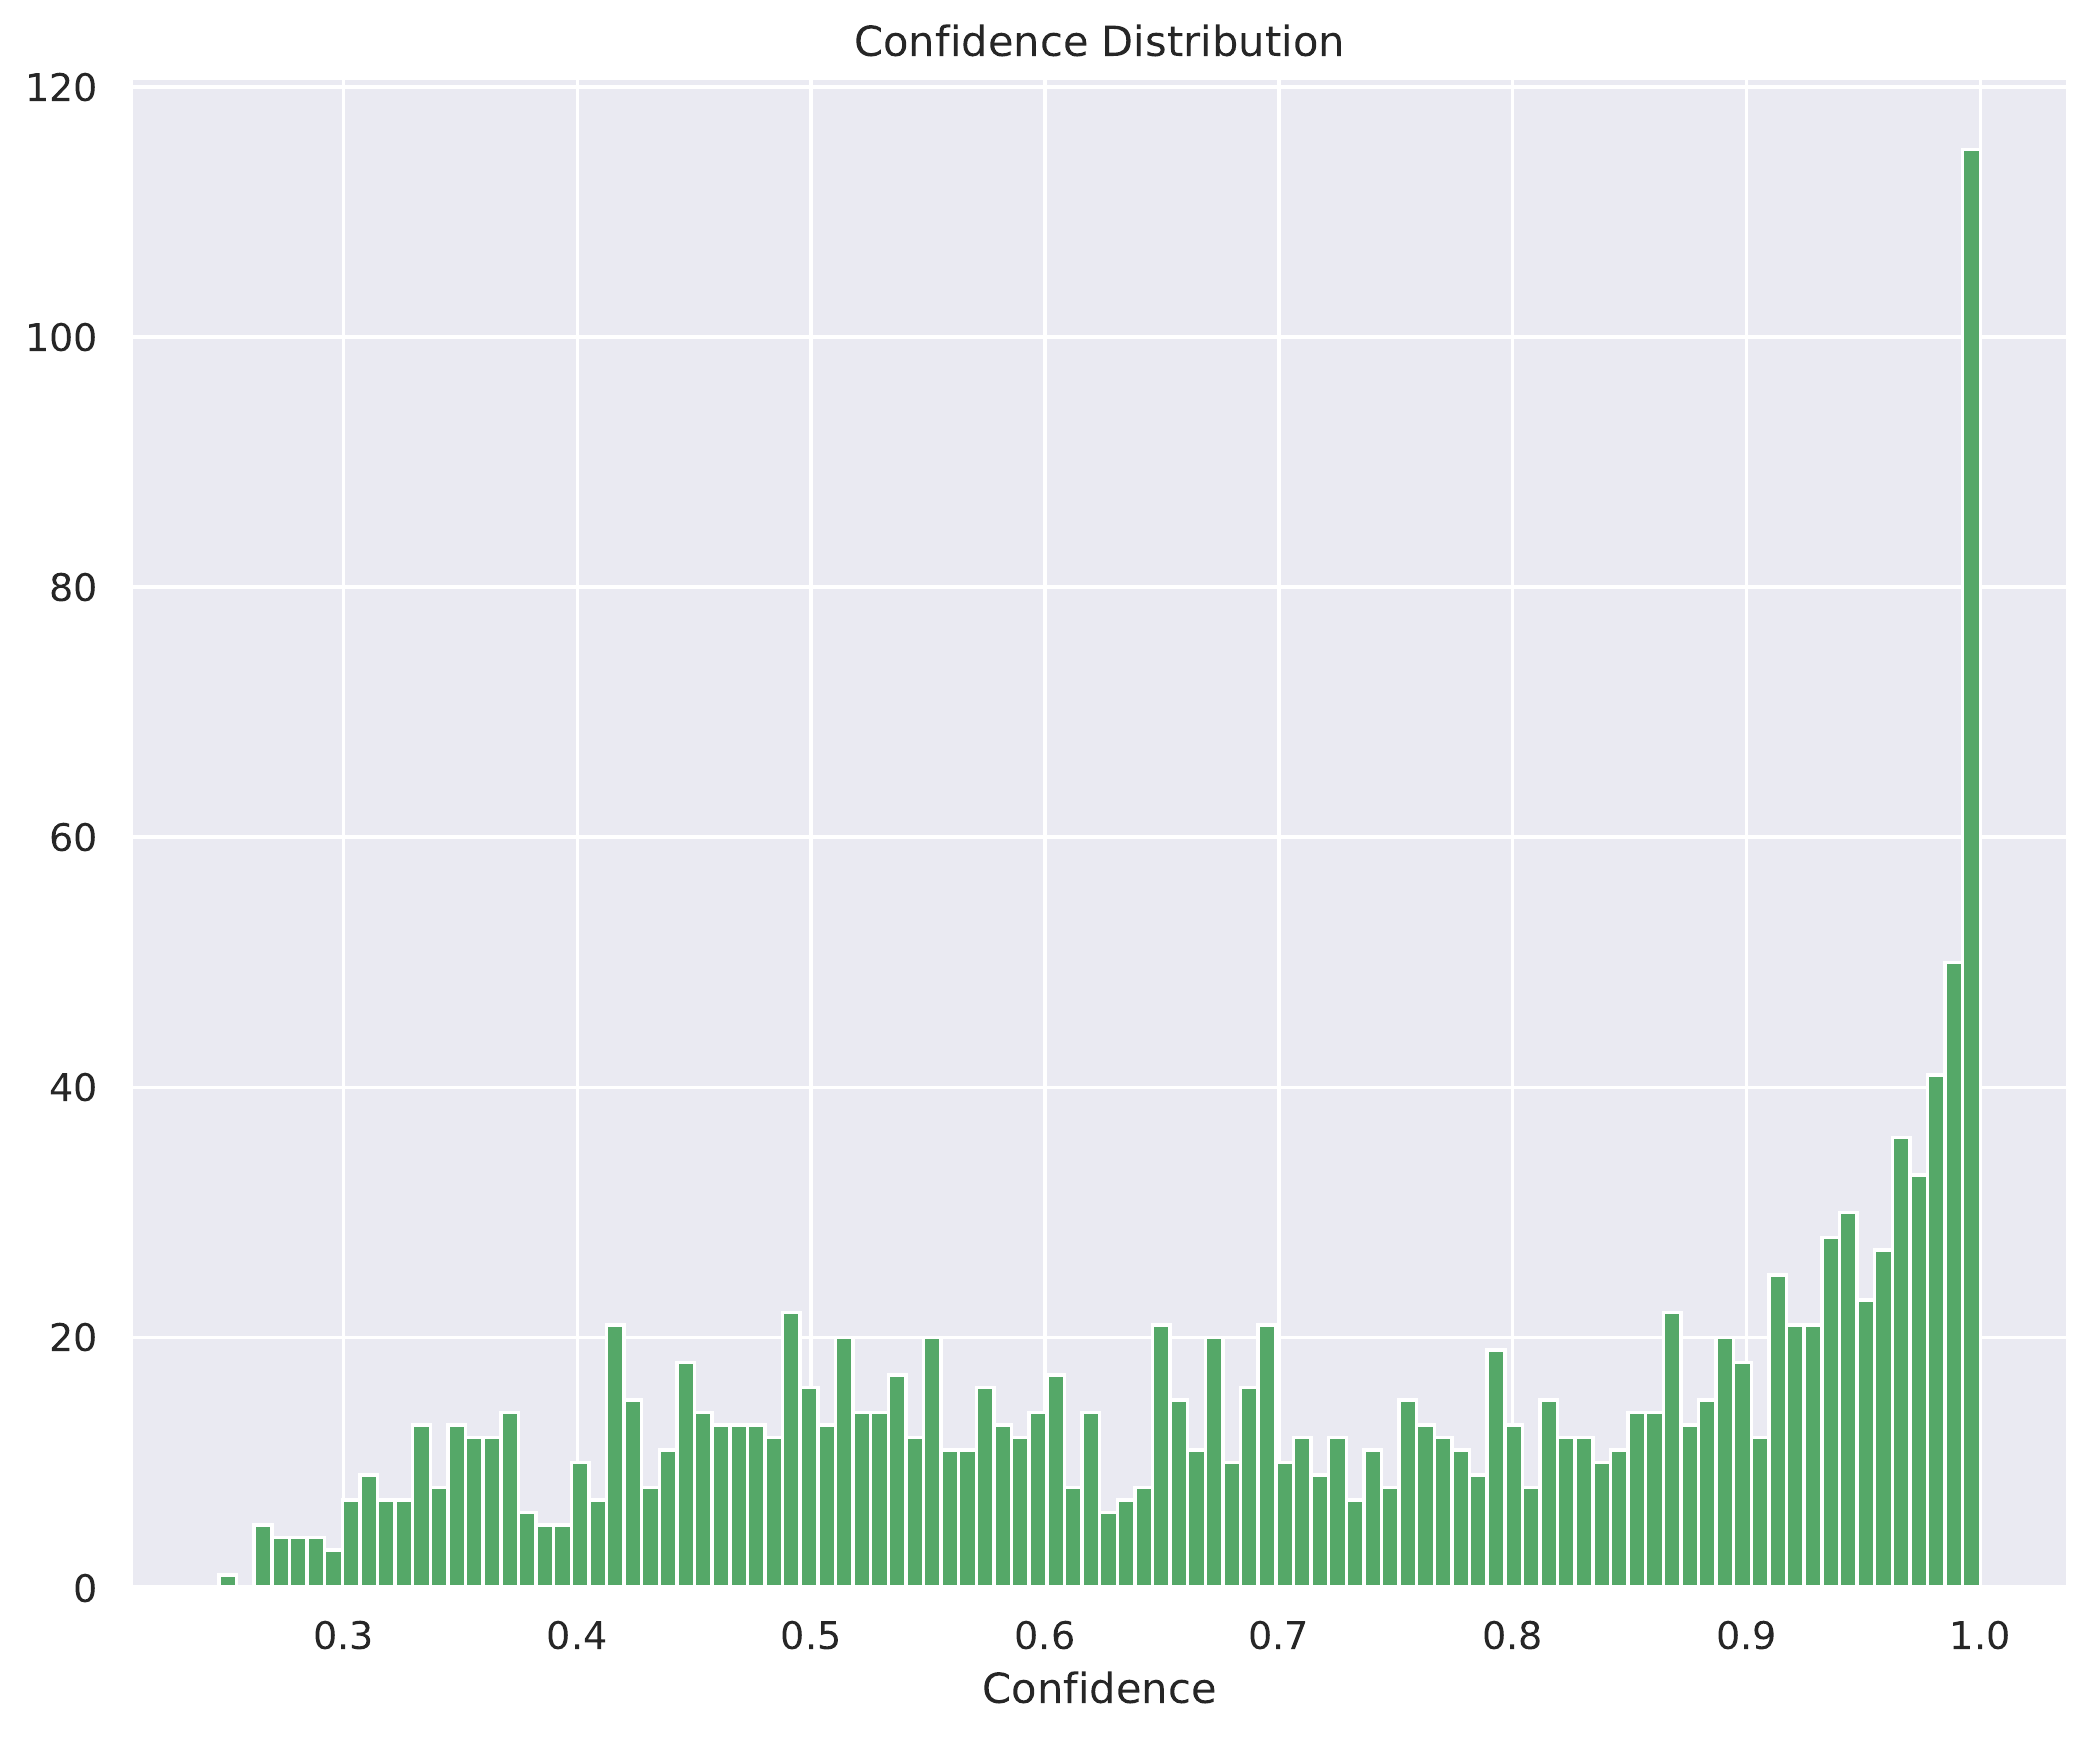} }}%
    \caption{Histogram of prediction confidence distribution on Citeseer dataset. The x-axis indicates the confidence of the model on the samples, and y-axis is the count on a normal scale of data points that fall into a given confidence bin. Left diagram is for GCN while right diagram is ouput of GPCN.}%
    \label{fig:conf_distribution_citeseer}%
\end{figure}

\begin{figure}[H]
    \centering
    {{\includegraphics[width=6.5cm]{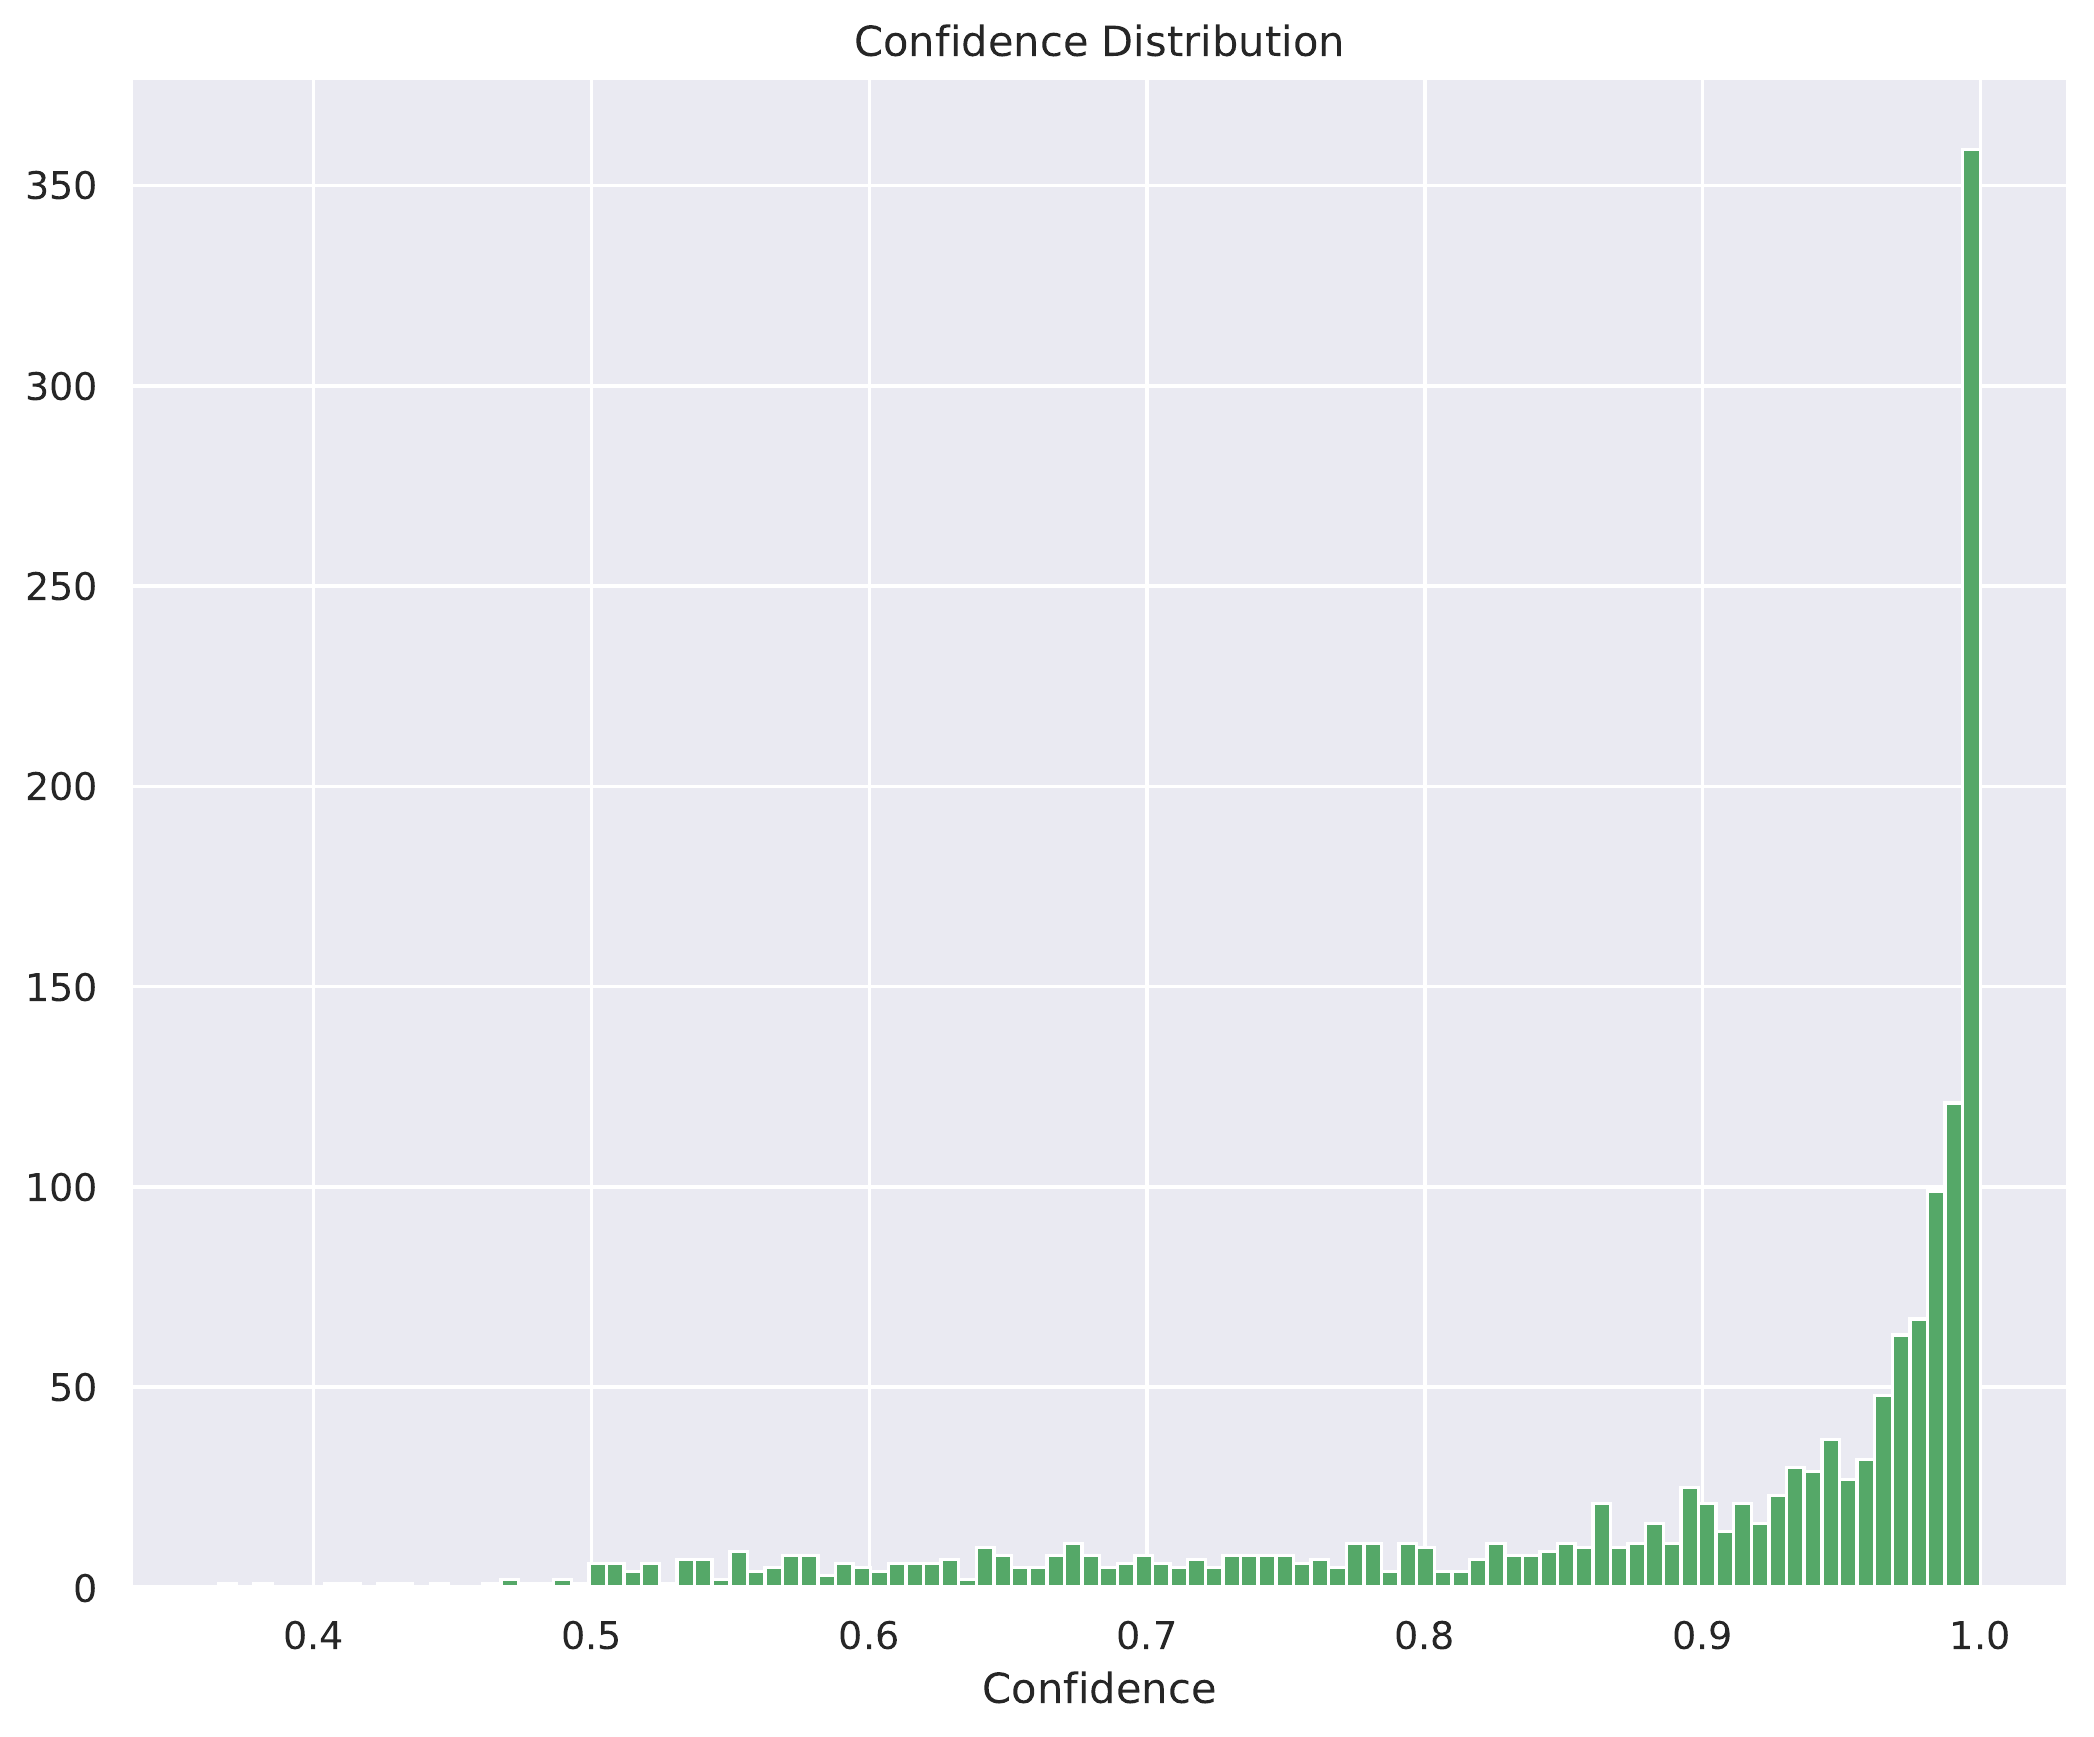} }}%
    \qquad
    {{\includegraphics[width=6.5cm]{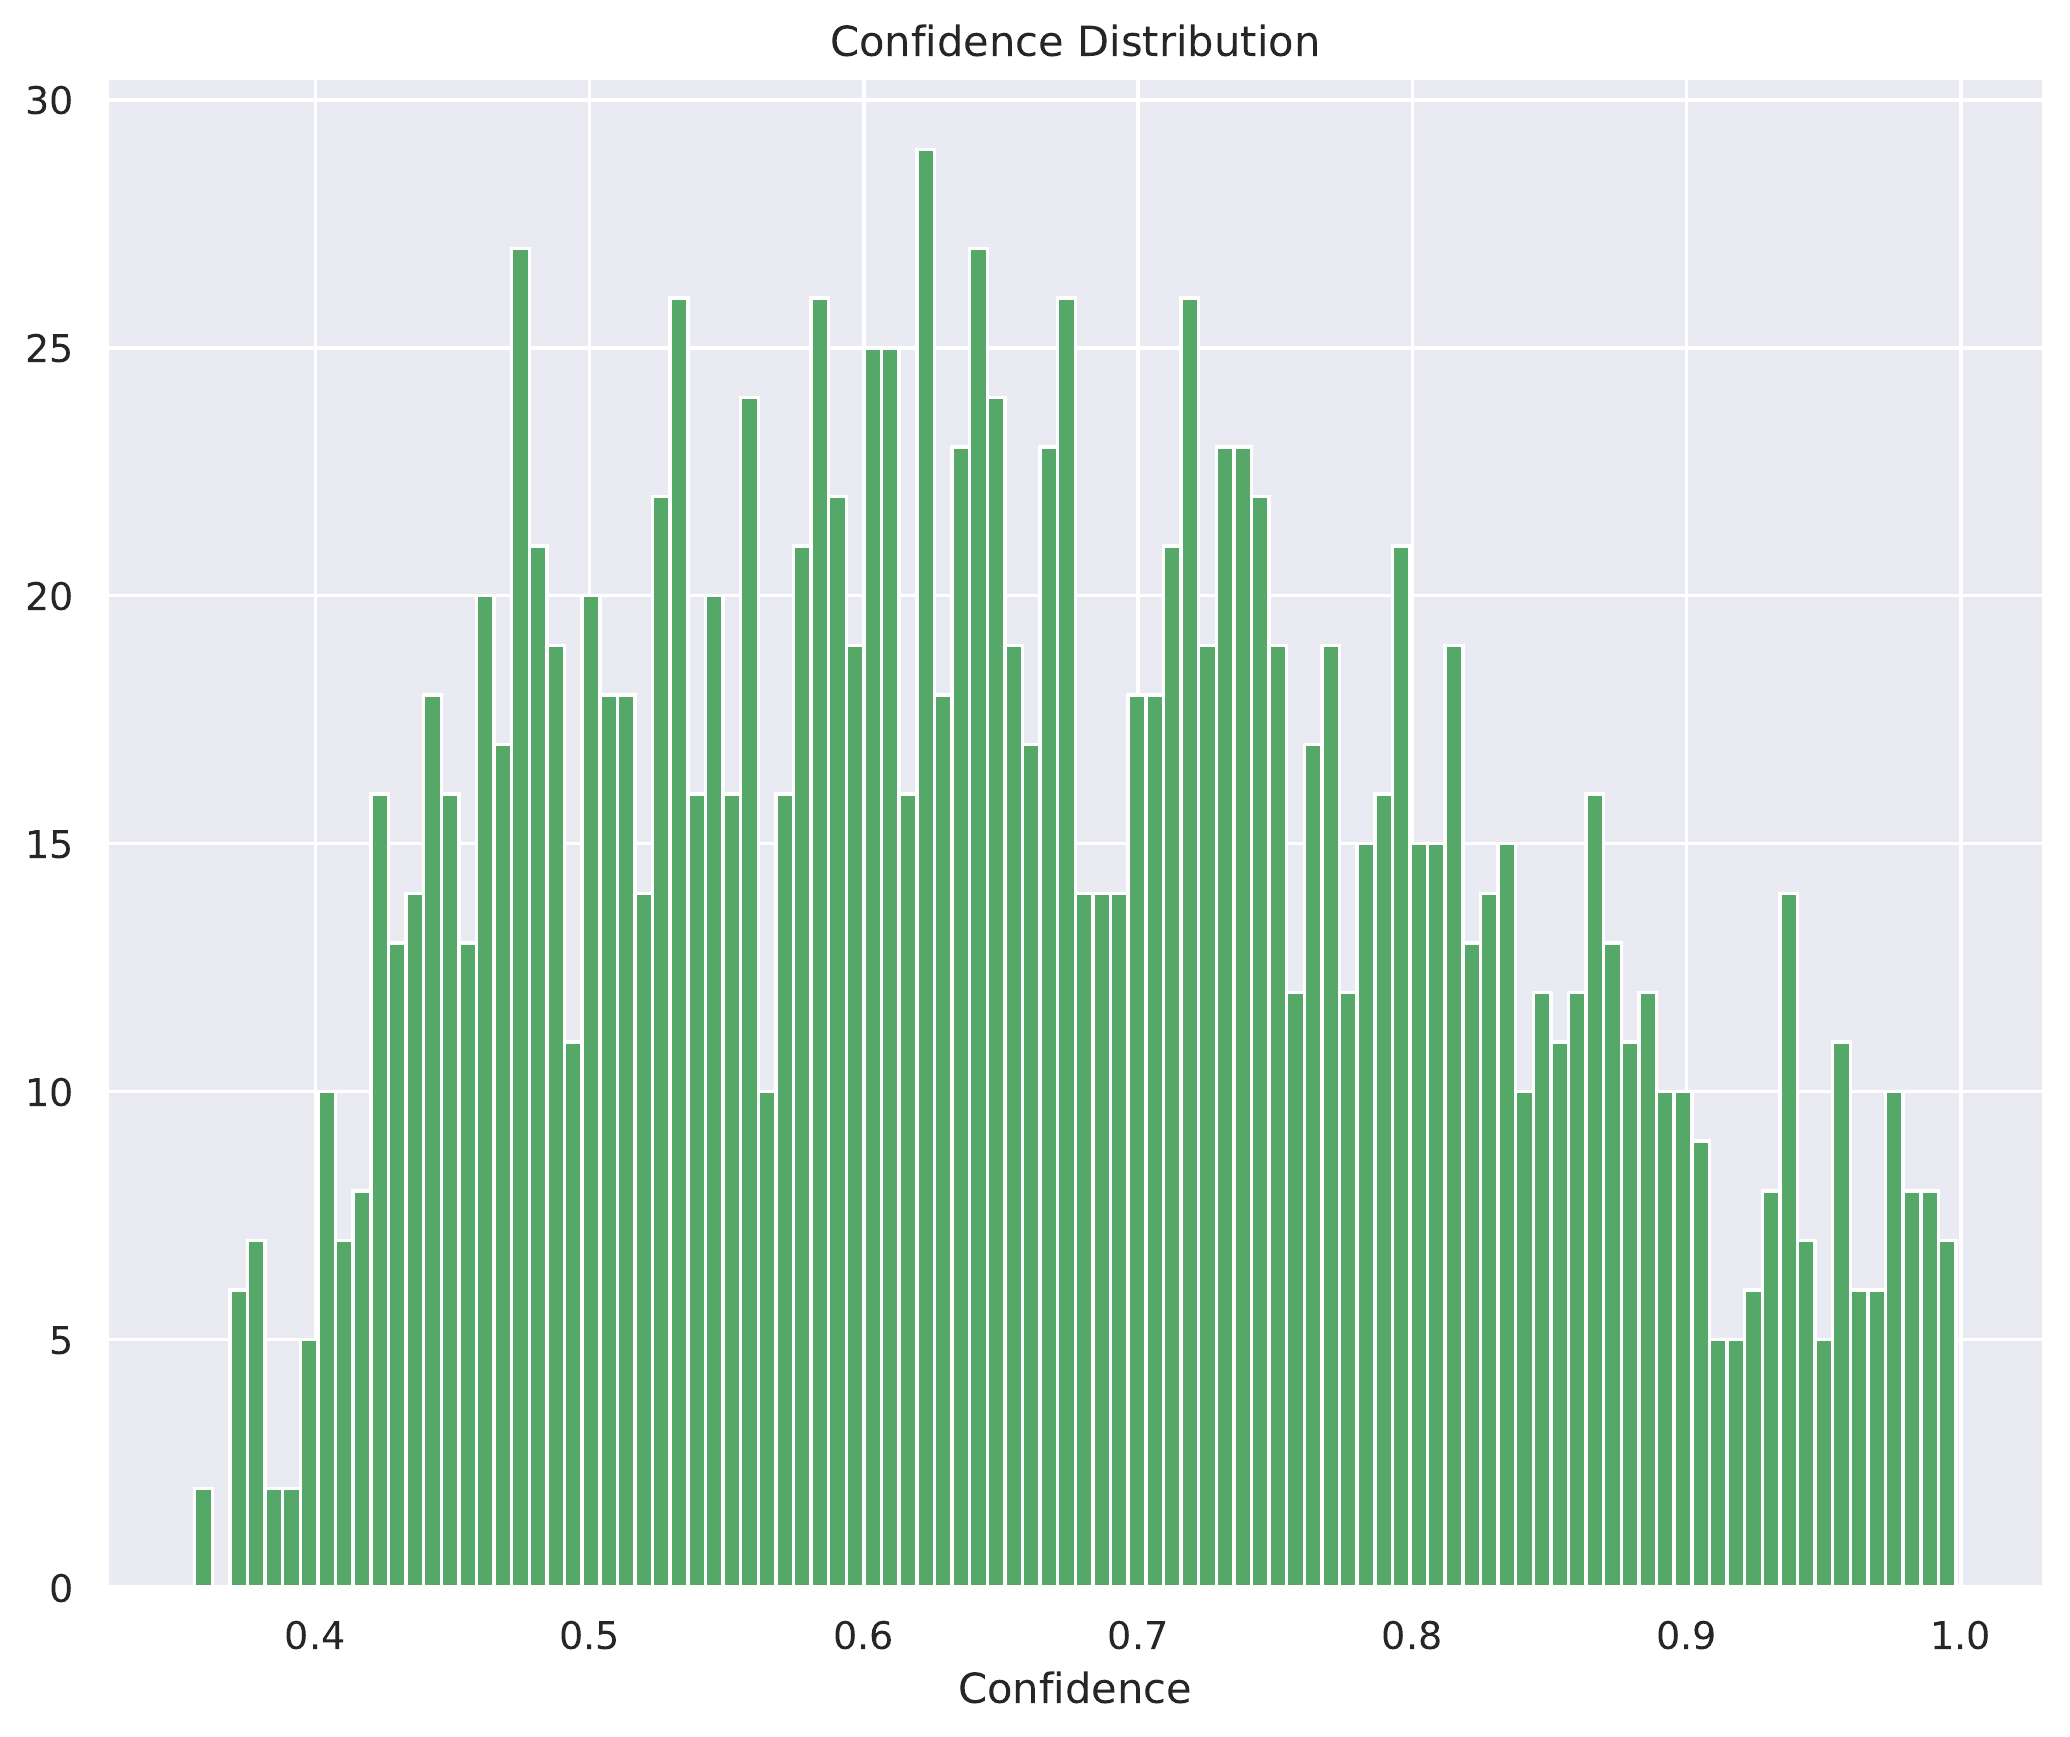} }}%
    \caption{Histogram of prediction confidence distribution on PubMed dataset. The x-axis indicates the confidence of the model on the samples, and y-axis is the count on a normal scale of data points that fall into a given confidence bin. Left: GCN. Right: GPCN.}%
    \label{fig:conf_distribution}%
\end{figure}

\subsection{Calibration Strengthening through Energy Minimization }

We observed a high positive correlation between calibration and training energy level, thus, we further investigated the role of energy to robustness and calibration of our learned representation. Unlike the standard predictive coding network, we observed, GPCN requires several inference steps to reach lowest training energy possible, i.e., this can seen as reaching local optimal of likelihood maximisation function. More importantly, we also observed that the lower the energy the better the calibration is, i.e., the better the model can estimate uncertainty in its prediction. Figure~\ref{fig:energy_calibration} on Cora dataset and Figure~\ref{fig:energy_calibration_citeseer} on CiteSeer dataset showcase this correlation. The plots on the left show that inference steps correlate to the energy level, i.e., the longer the inference is, the more likely that the model converge to a lower energy. The middle diagram and right diagrams, similarly, present the correlation between the inference steps and ECE and MCE, respectively, which from left diagrams, implies the correlation of energy level and ECE and MCE. We see that the lower the energy the better the calibration performance reached.

As it has been shown that calibration can be affected by learning rates \cite{guo2017calibration}, we track the ECE and MCE throughout training, and we see that as the lower the learning rate, the better and more stable calibration GPCN is able to attain based on ECE and MCE metrics (see Figure ~\ref{fig:ece_lr} and \ref{fig:mce_lr}).

\begin{figure}[H]
    \centering
    \makebox[\textwidth]{
    \includegraphics[width=12cm]{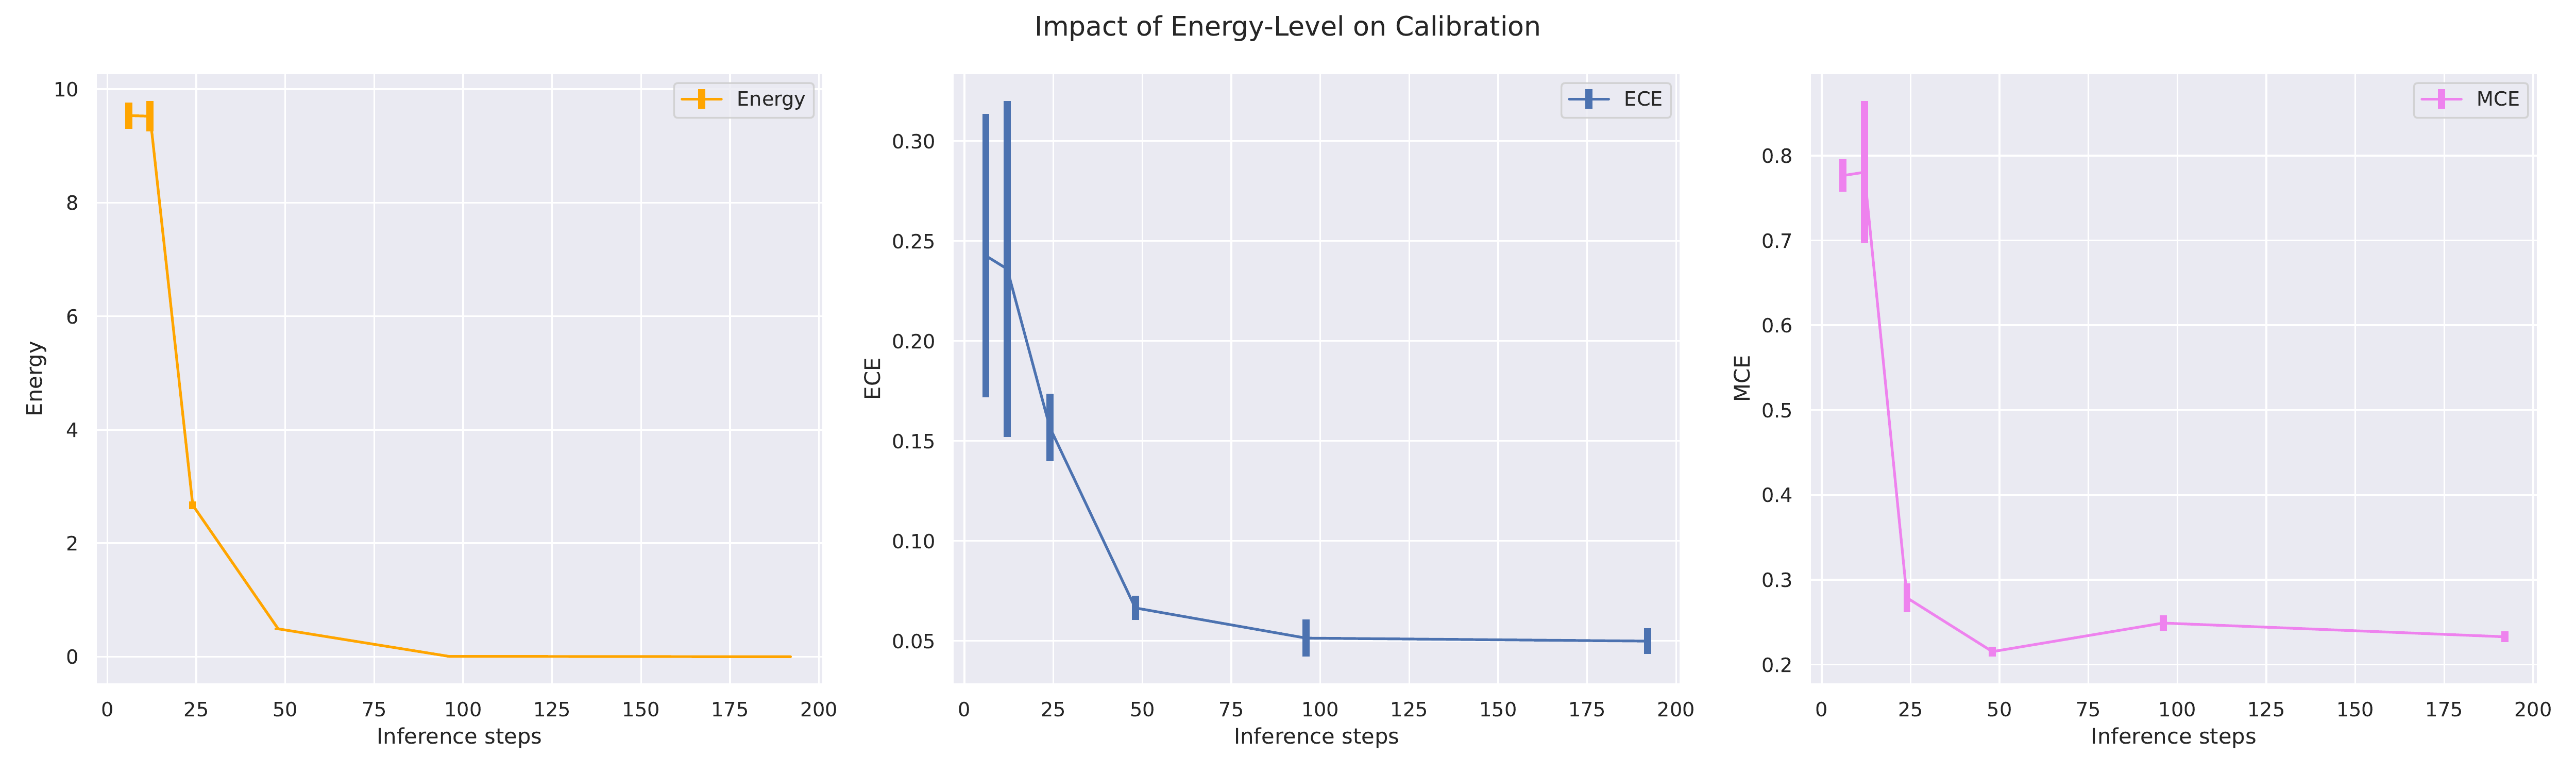}
    }
    \caption{Evaluation of the impact of energy on  calibration performance on Cora dataset (learning rate $= 0.001$). Left: Demonstrates that increasing inference steps leads to lower energy. Middle: Shows that the lower energy level determines expected error(ECE). Right: Also showcase, the correlation between energy and maximum calibration error(MCE)}
    \label{fig:energy_calibration}
\end{figure}

\begin{figure}[H]
    \centering
    \makebox[\textwidth]{
    \includegraphics[width=12cm]{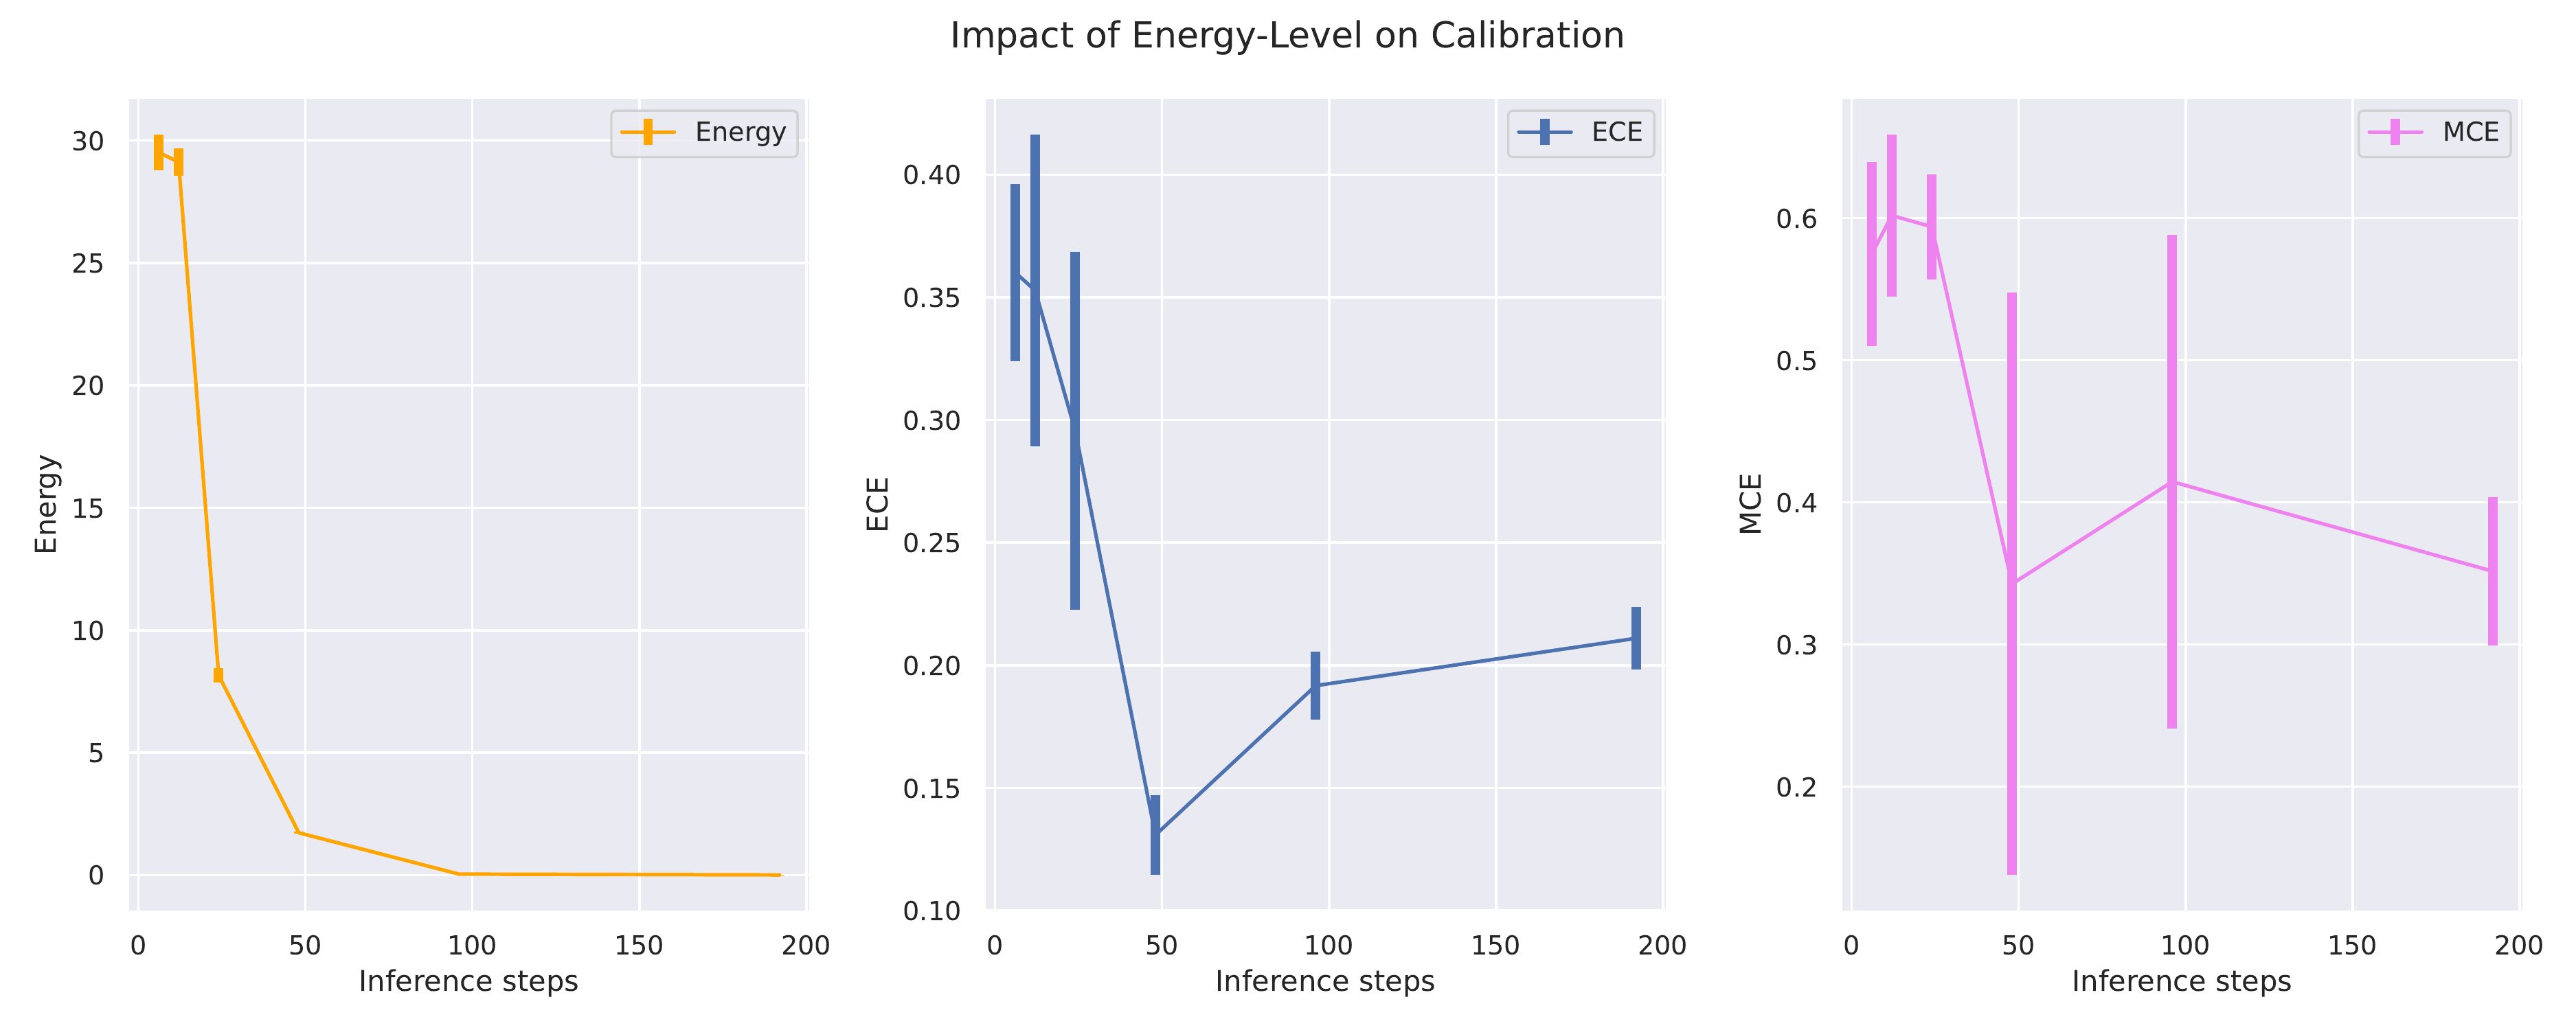}
    }
    \caption{Evaluation of the impact of energy on  calibration performance on CiteSeer dataset. Left: Demonstrates that increasing inference steps leads to lower energy. Middle: Shows that the lower energy level determines expected error(ECE). Right: Also showcase, the correlation between energy and maximum calibration error(MCE)}
    \label{fig:energy_calibration_citeseer}
\end{figure}

\begin{figure}
    \centering
{{\includegraphics[width=6.5cm]{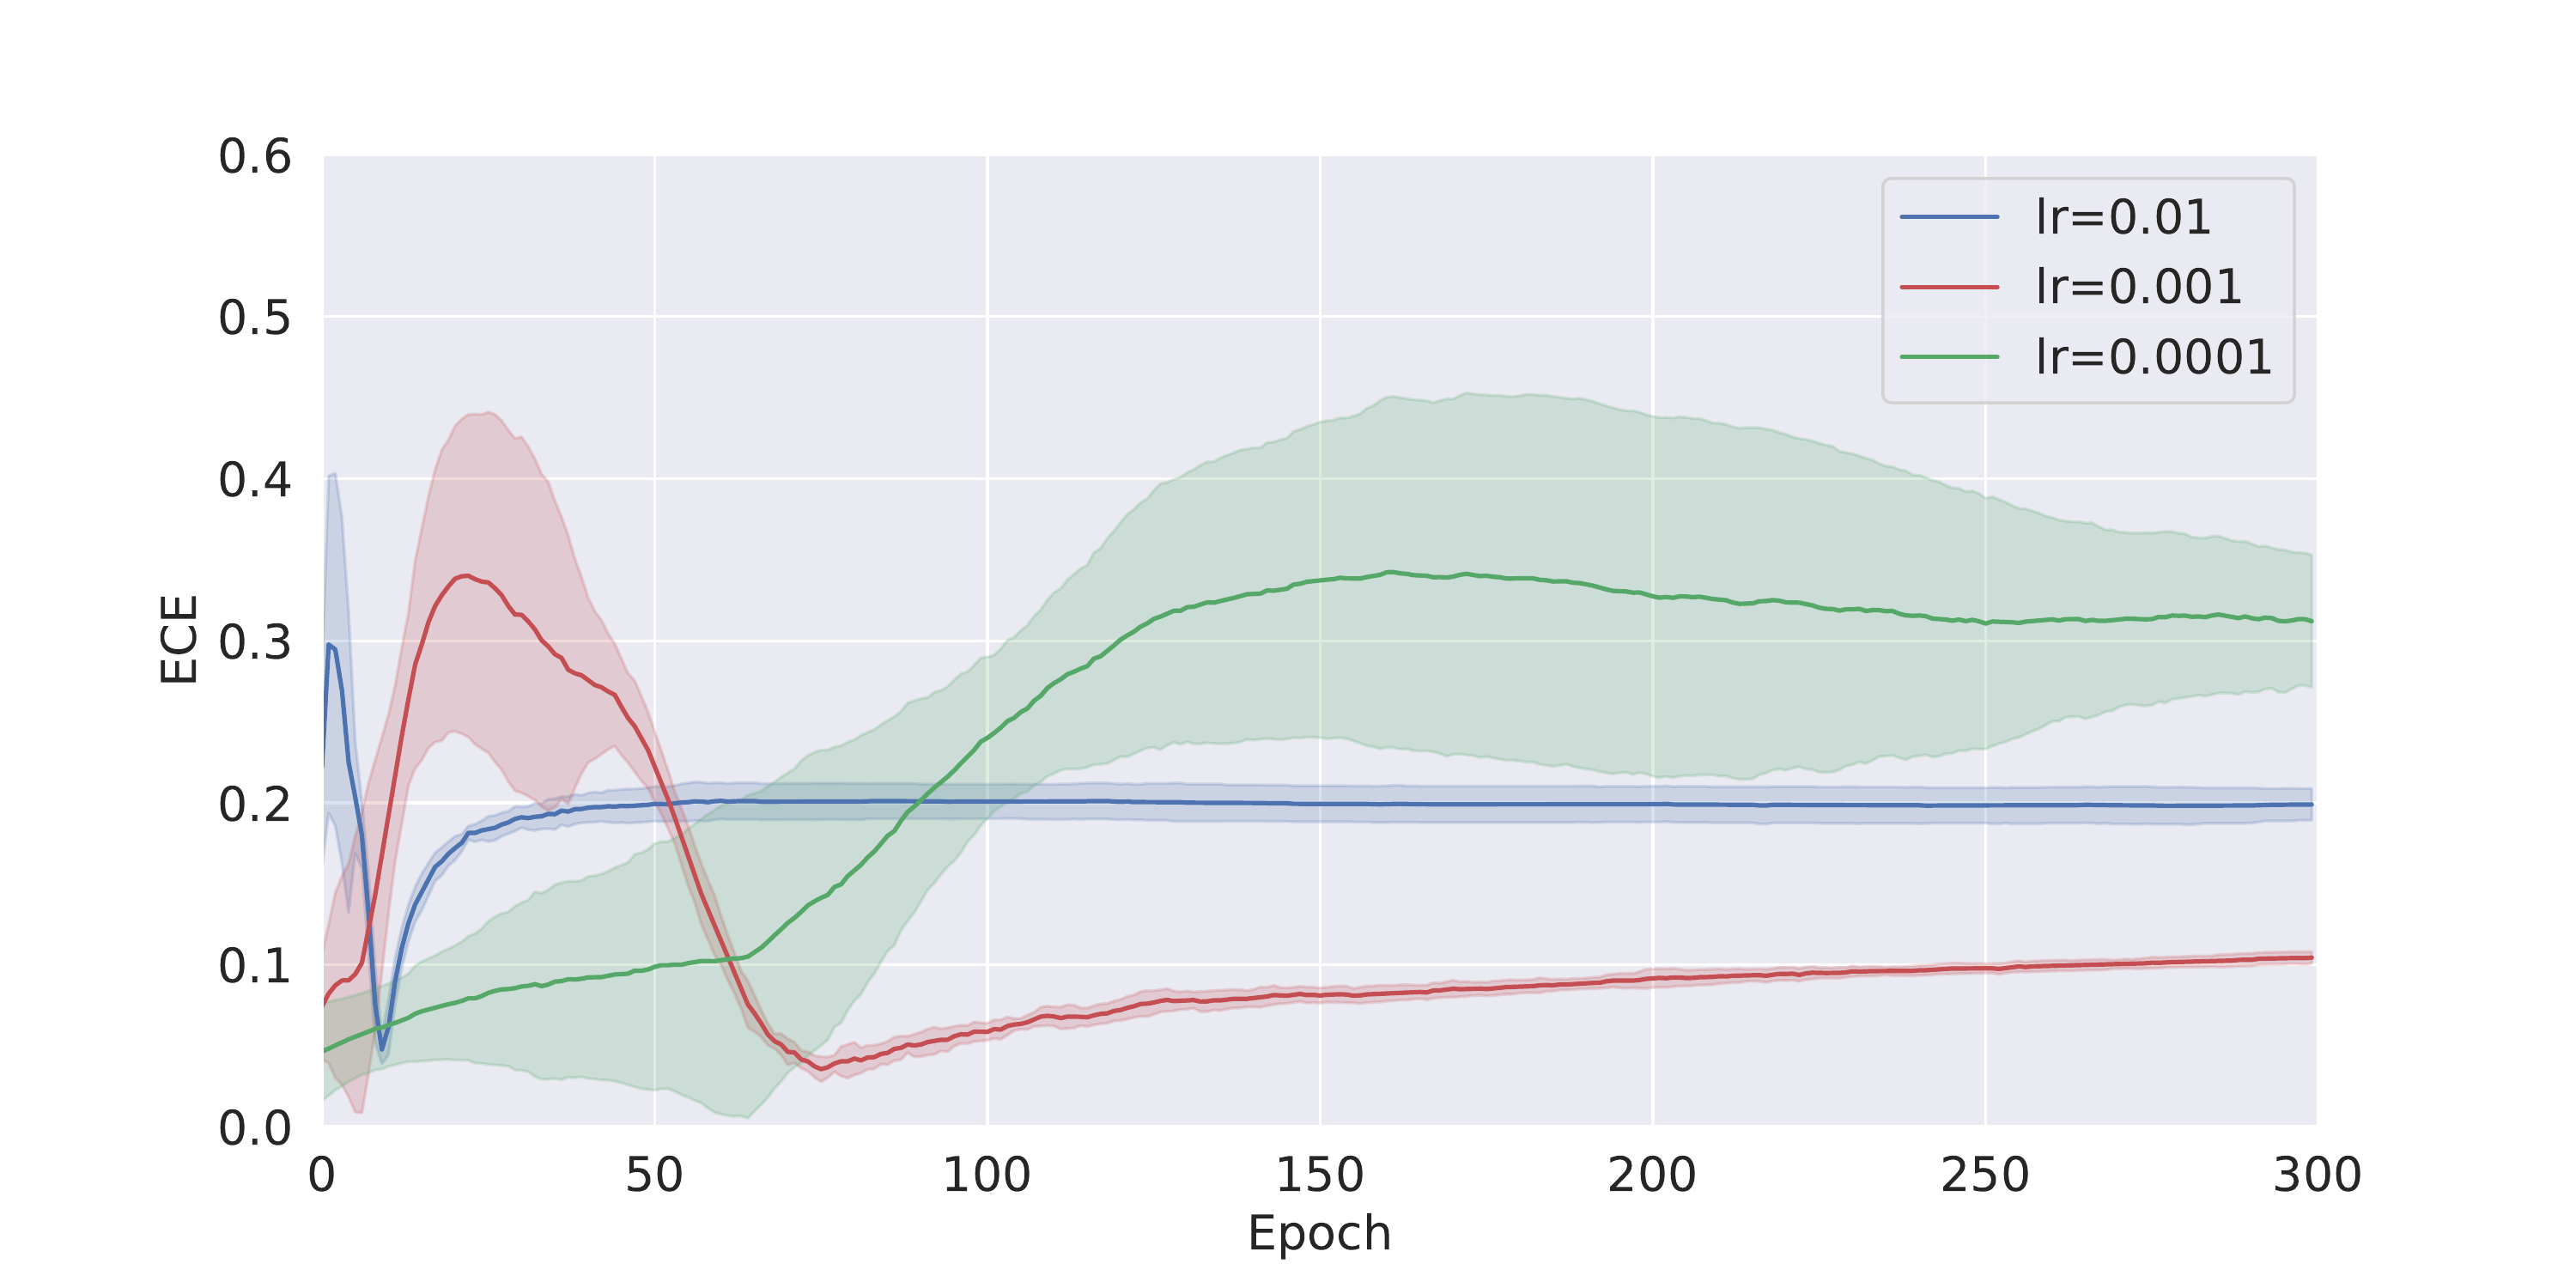} }}%
    \qquad
    {{\includegraphics[width=6.5cm]{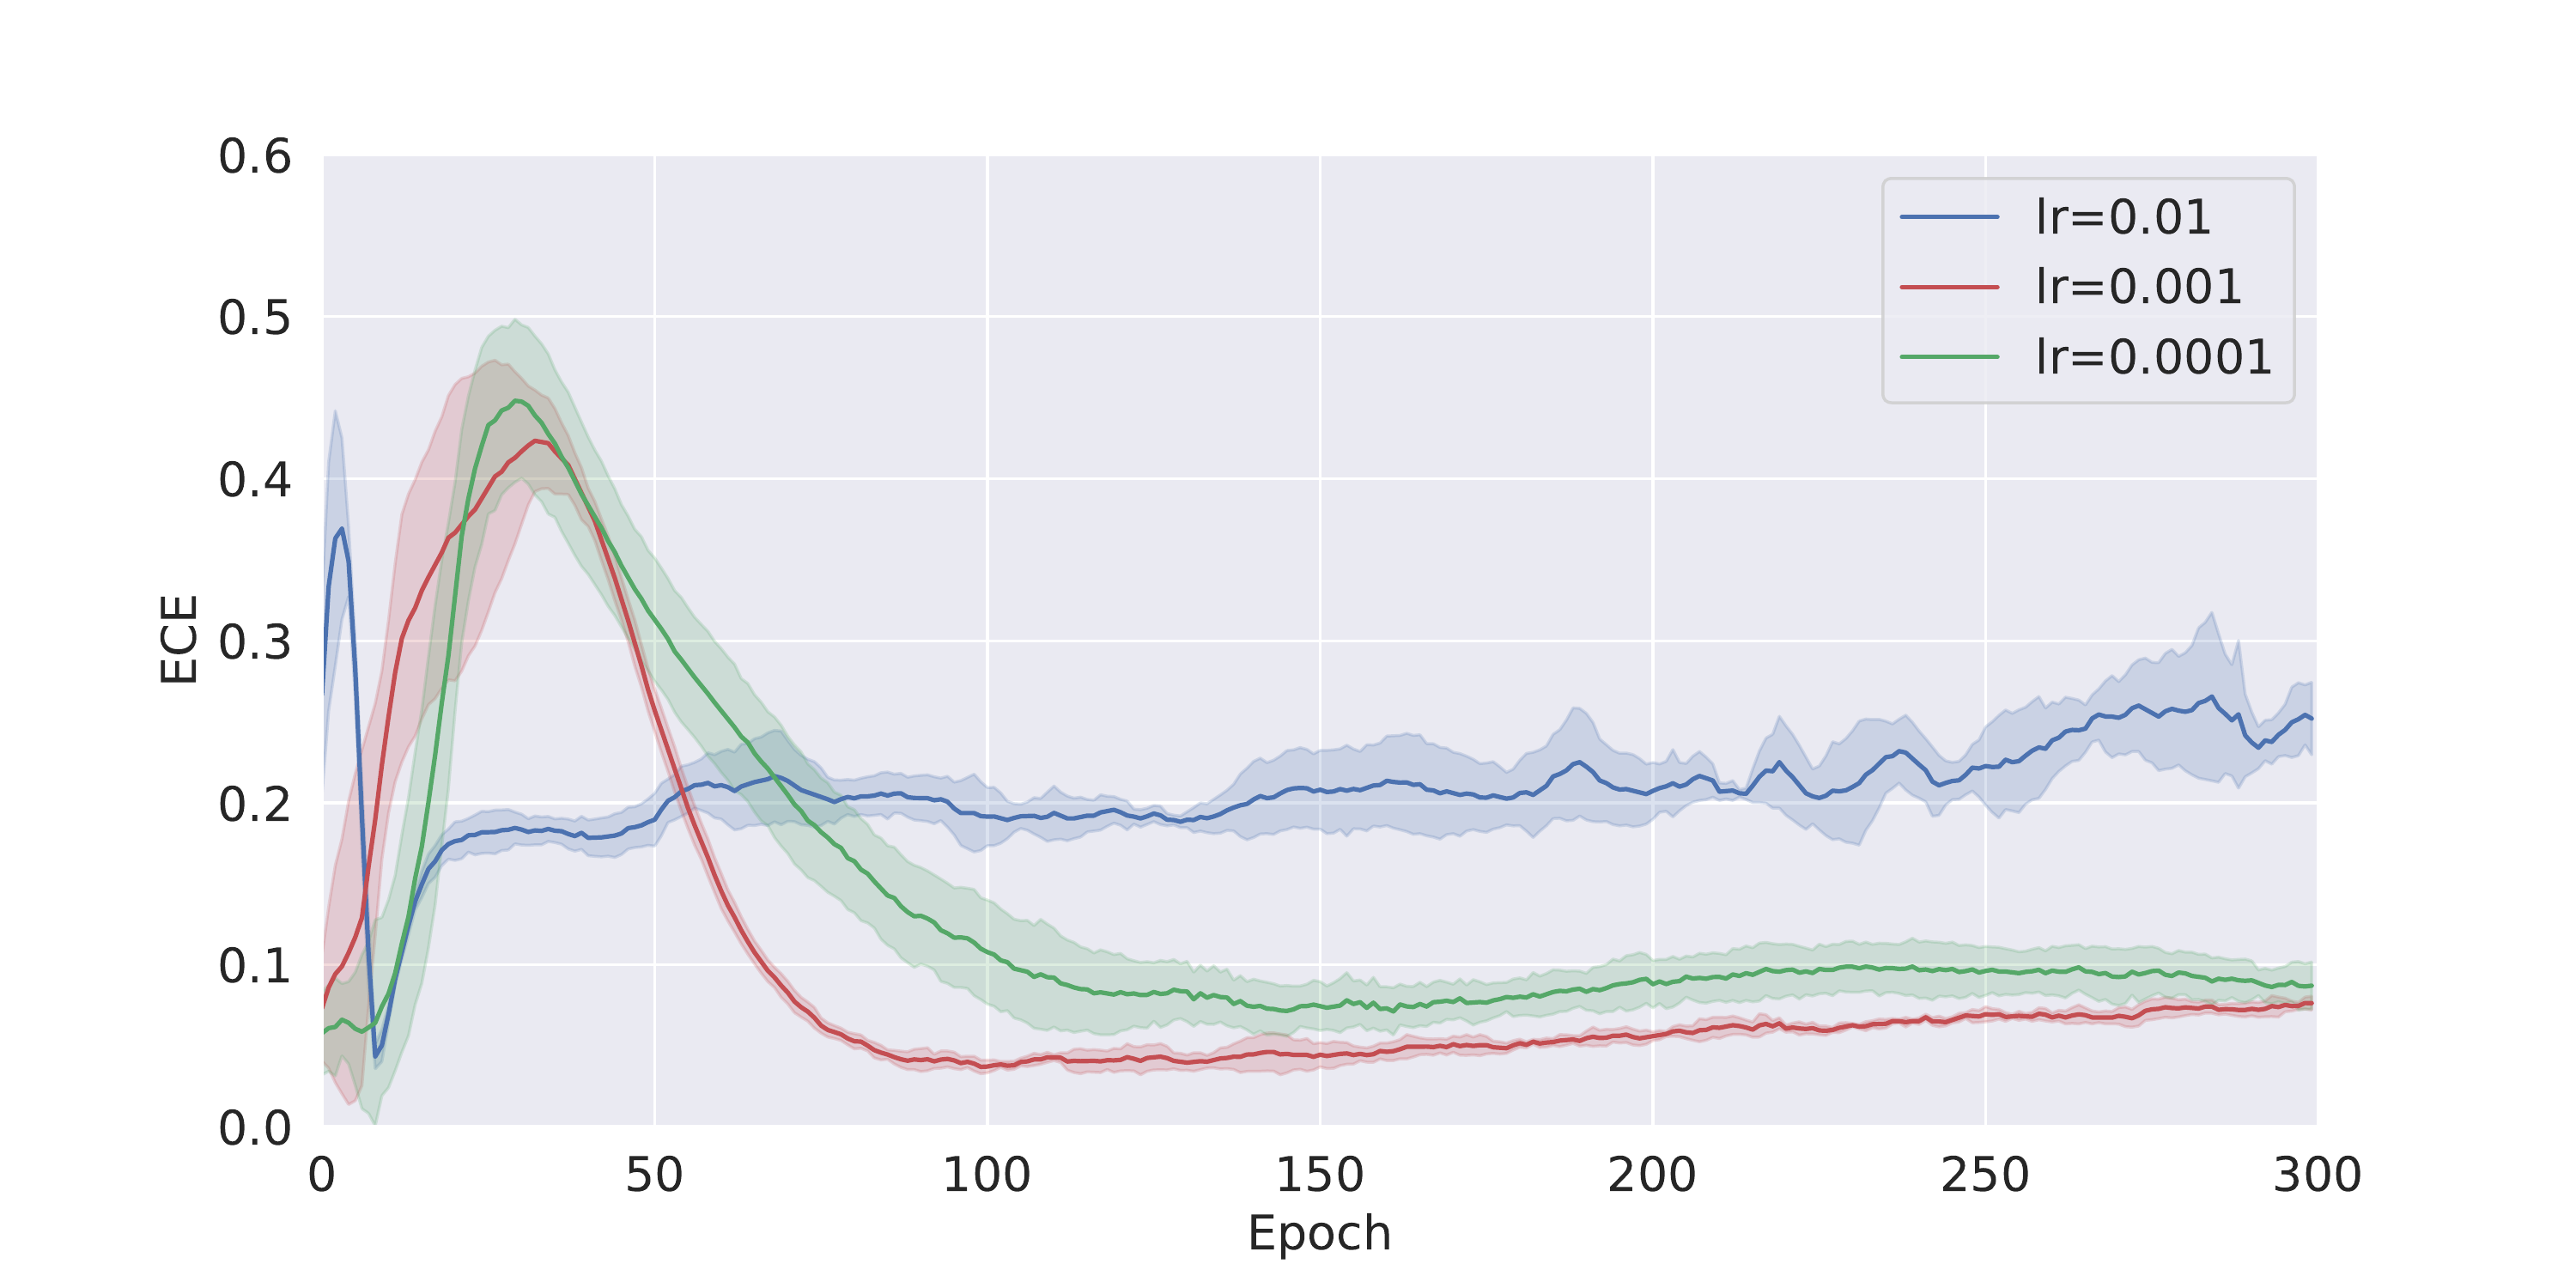} }}%
    \caption{Evolution of expected calibration error (ECE) on test set during training on various learning rates (lr). Left: GCN. Right: GPCN.}%
    \label{fig:ece_lr}%
\end{figure}

\begin{figure}
    \centering
{{\includegraphics[width=6.5cm]{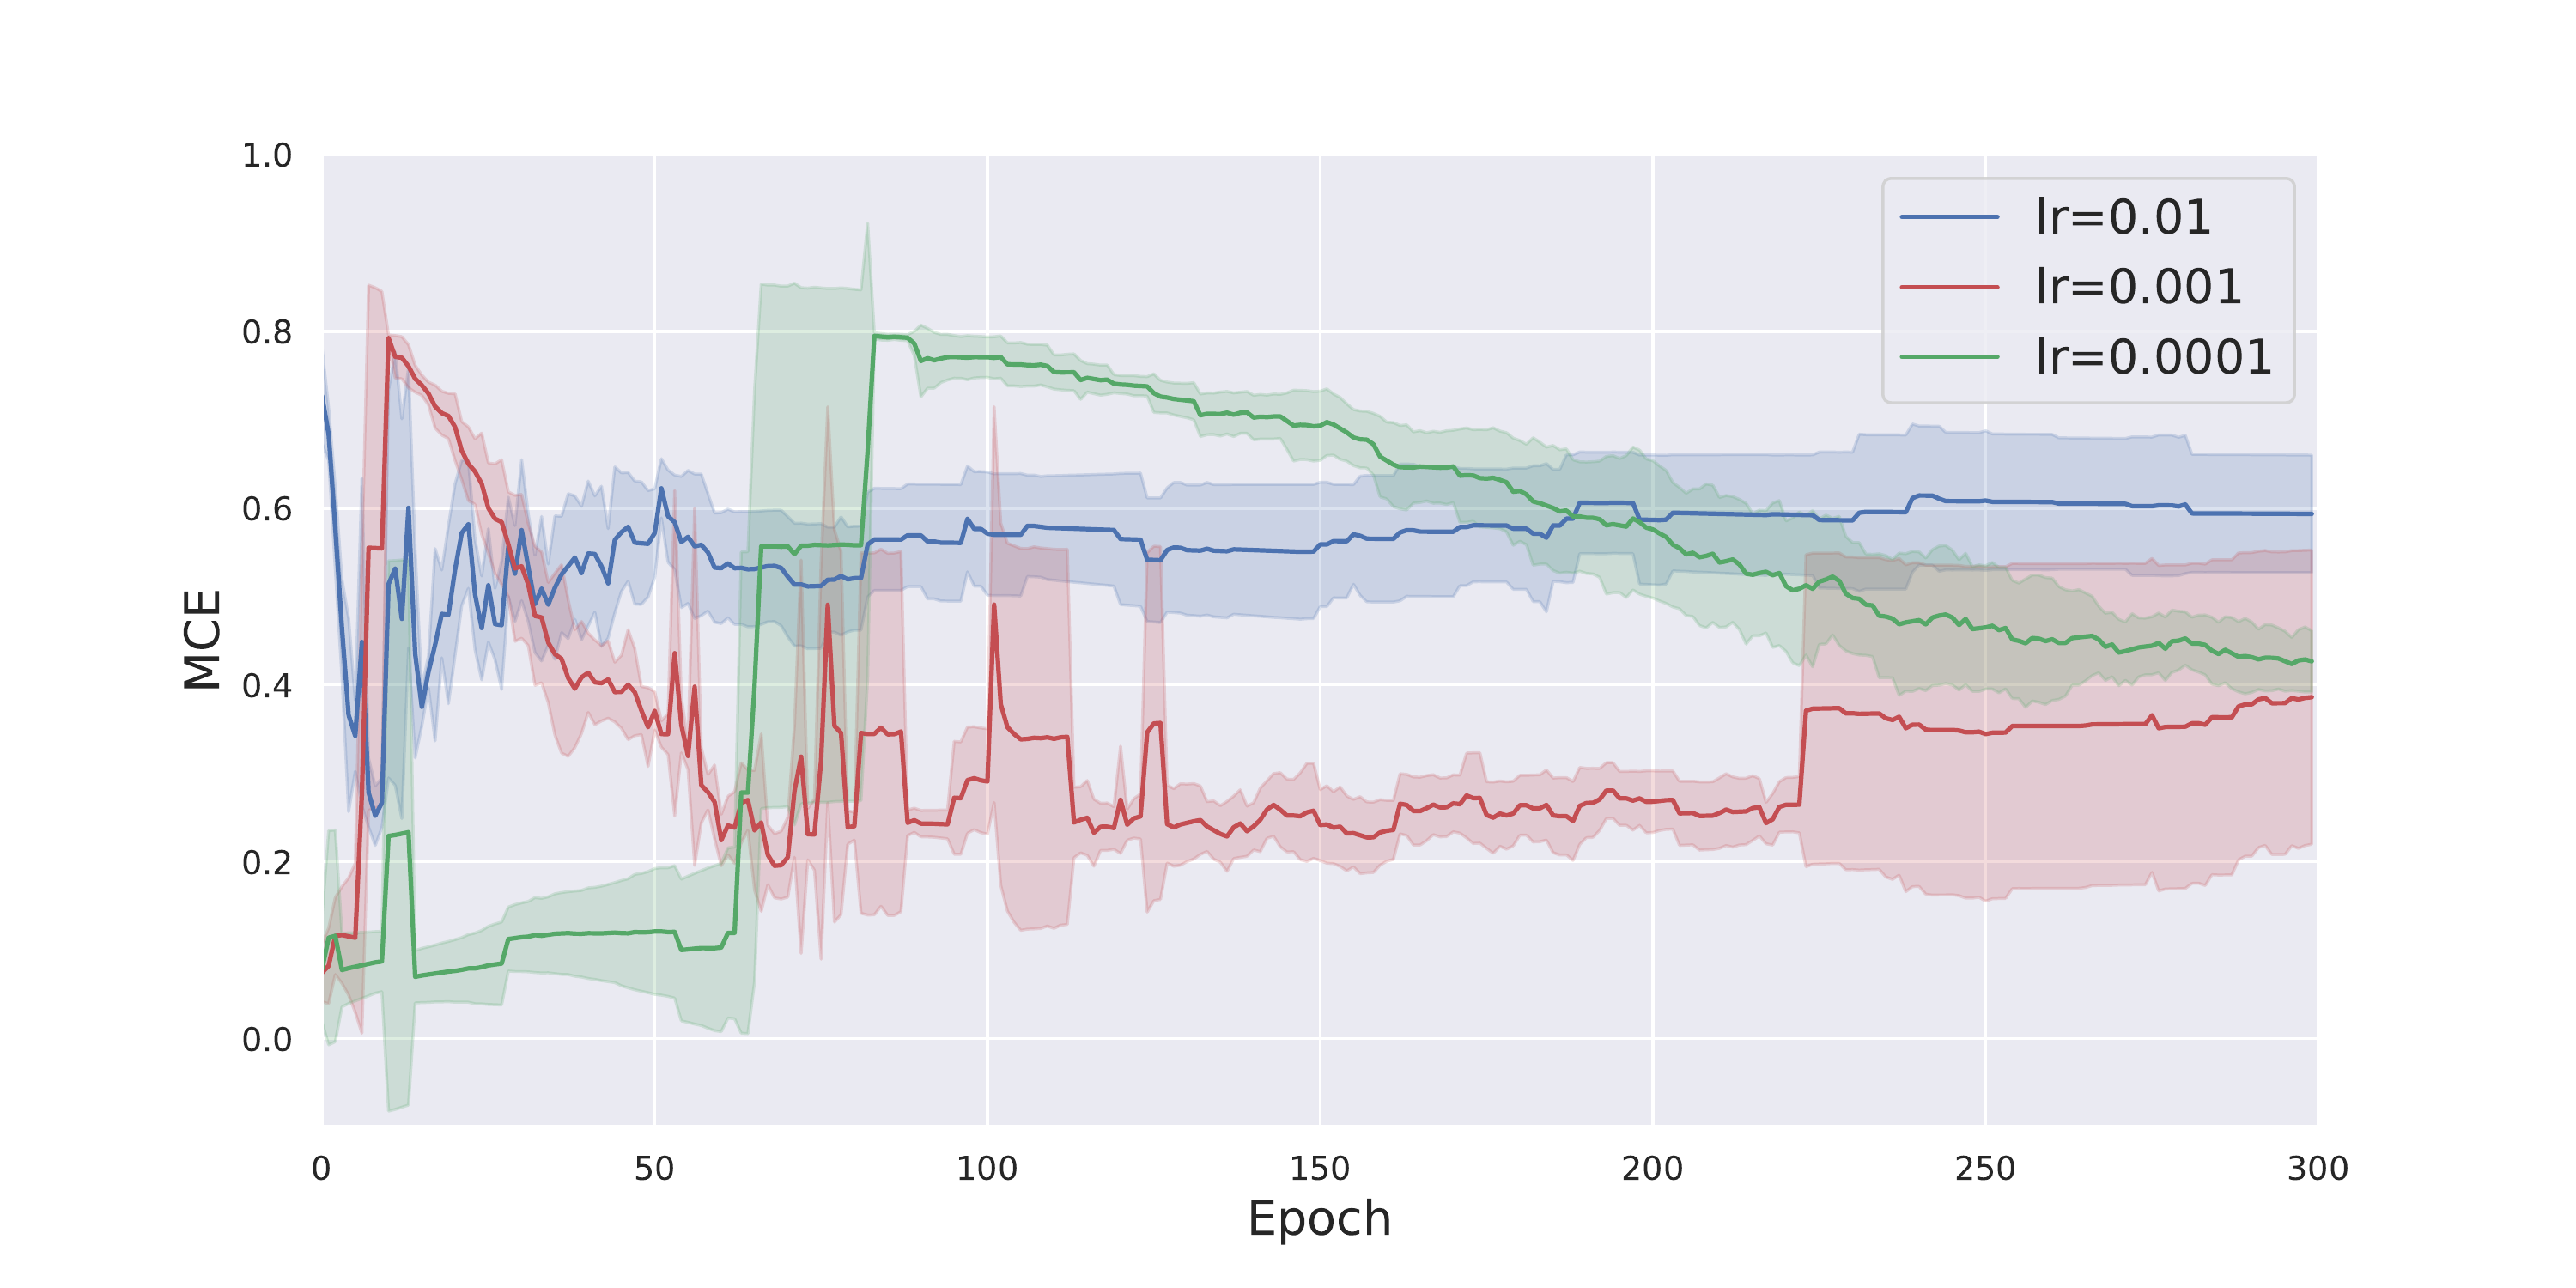} }}%
    \qquad
{{\includegraphics[width=6.5cm]{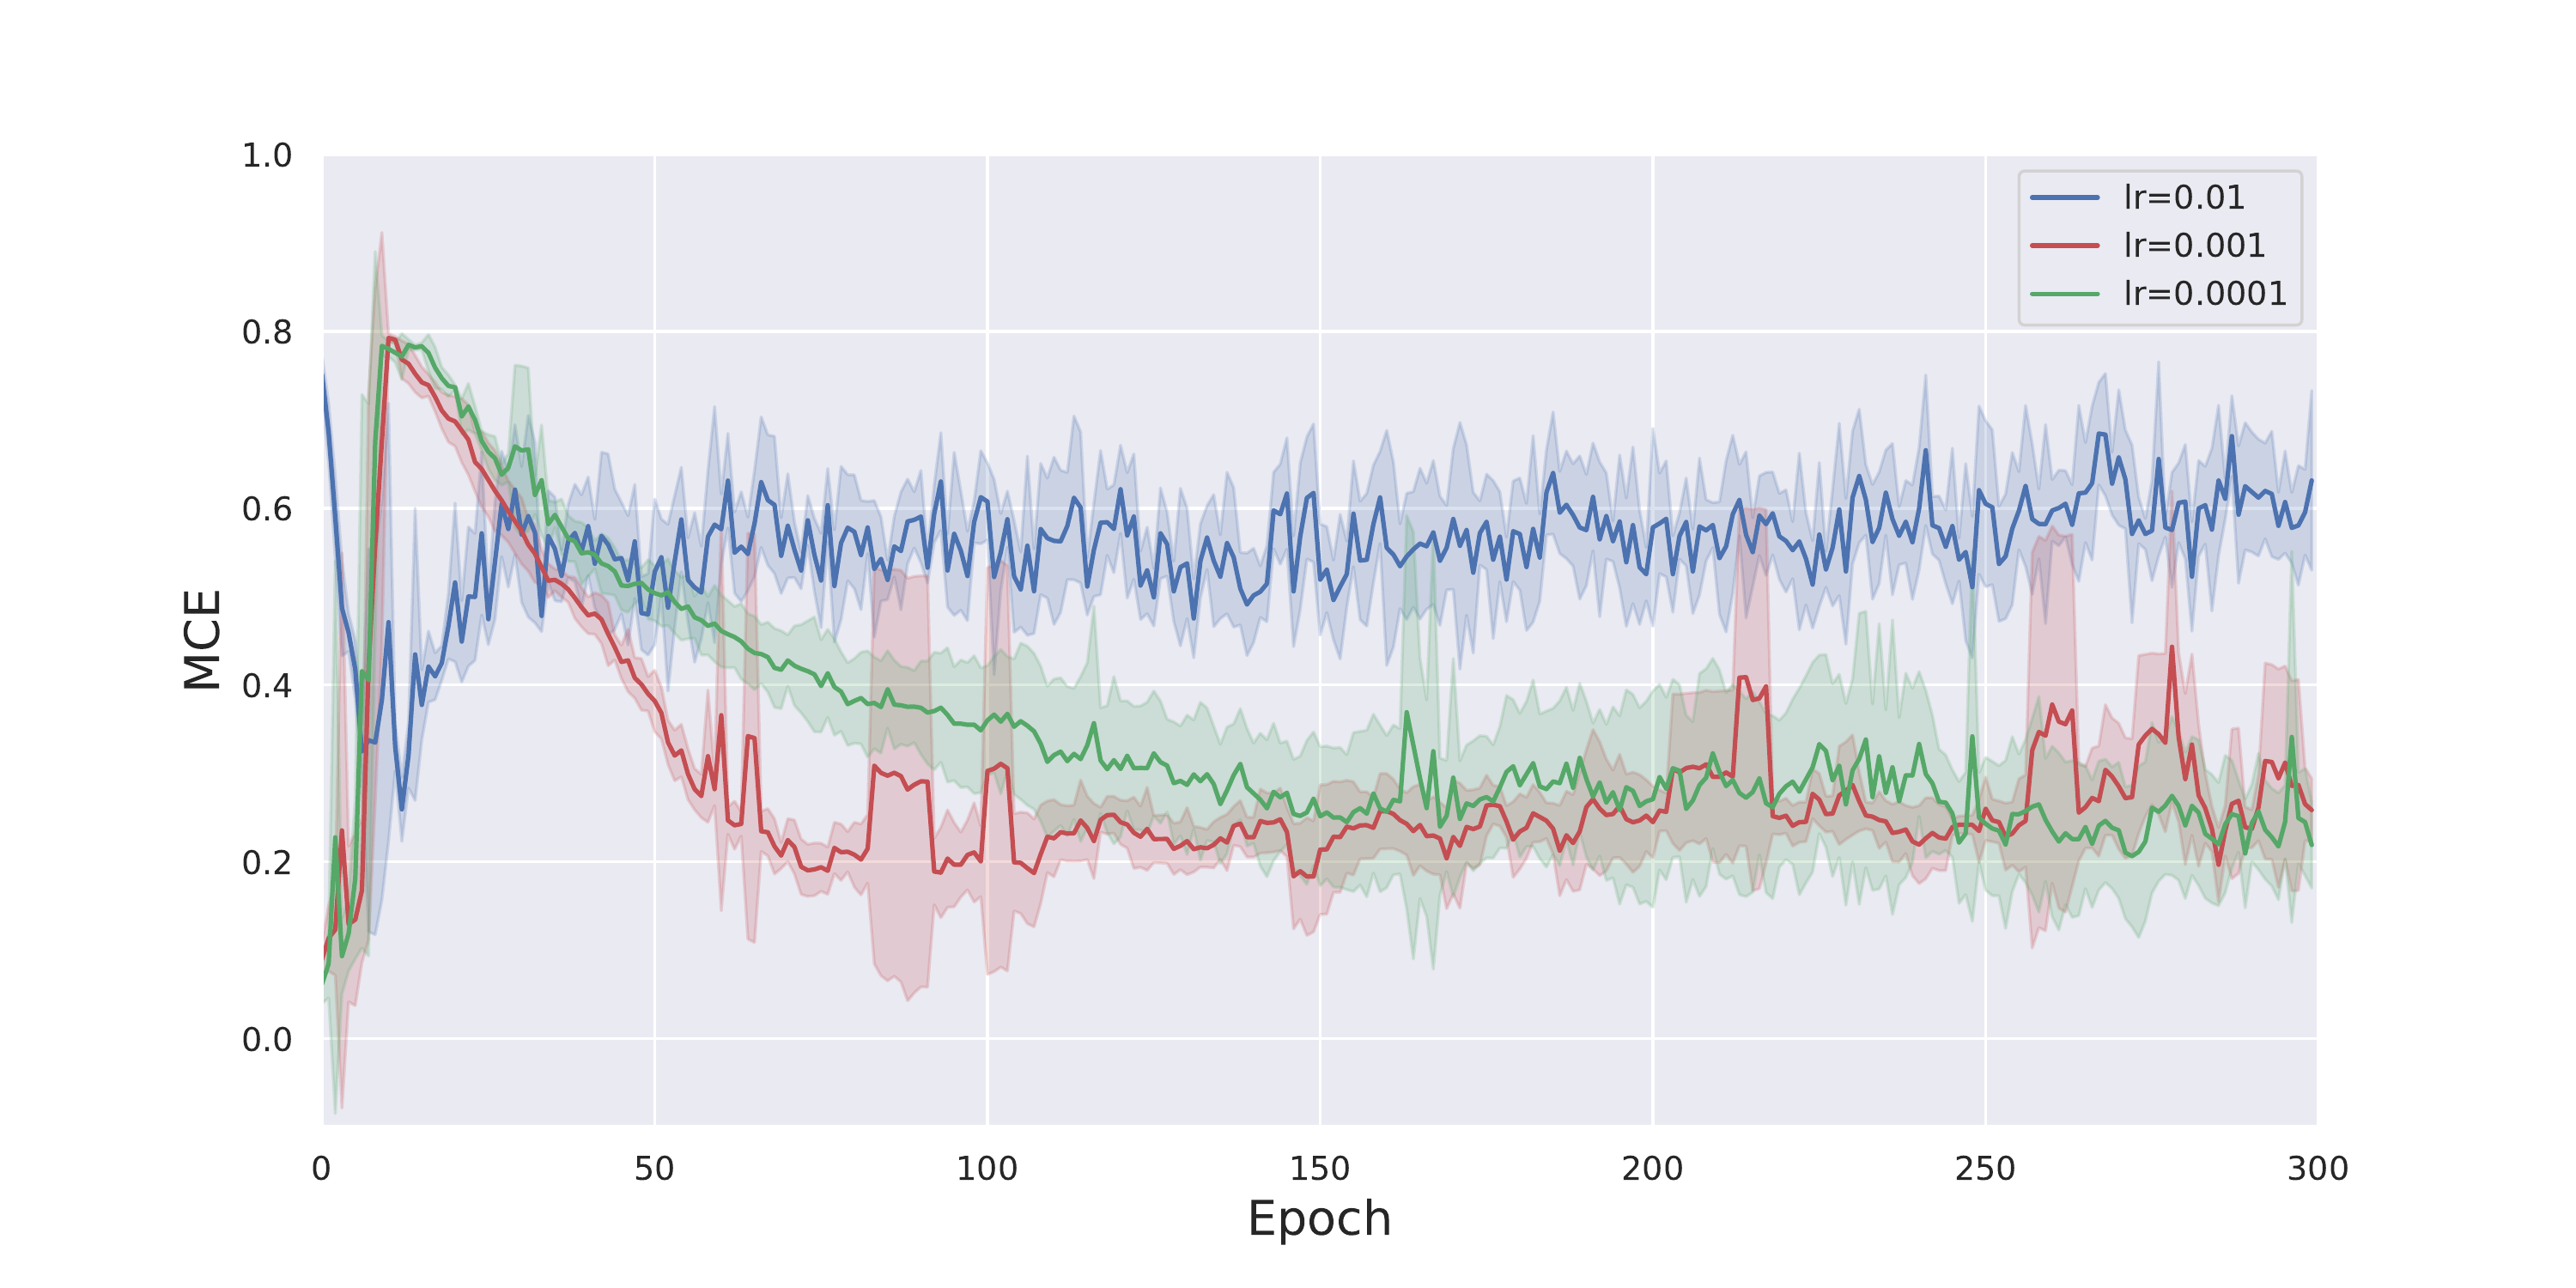} }}%
    \caption{Evolution of maximum calibration error (MCE) on test set during training on various learning rates (lr). Left: GCN. Right: GPCN.}%
    \label{fig:mce_lr}%
\end{figure}

\section{GPCN architecture}

Using a simple graph in Figure~\ref{fig:example_graph}, here, we demonstrate the idea of graph predictive coding as opposed to standard graph neural networks. In typical graph convolution network (GCN) \cite{welling2016semi} models, the node representation is obtained by the recursive aggregation of representations of its neighbours, after which a learned linear transformation and non-linear activation function are applied. After the $k_th$ round of aggregation (with $k$ denoting the number of GCN layer), the representation of a node reflects the underlying structure of its nearest neighbours within $k$ hops. Note that the GCN is one of the simplest GNN model, as the update function equates to only neighbourhood aggregation, that is why in Figure~\ref{fig:graph_mesage_passing}(left) we only depict the aggregate function as it captures the update function altogether. 

Our GPCN model (see Figure~\ref{fig:graph_mesage_passing}(right)) differs from the standard GNN in three aspects. First, node representation are not a mere result of neighborhood aggregation. Rather, each node has unique a neural state that is updated through energy-minimization using the theory of predictive coding described in the main body of this work. Specifically, each neighborhood aggregation at each hop, k,, pass through a predictive coding module that predicts the the incoming aggregated neighborhood representation. Second, GPCN has a different concept of what neighborhood messages are (see Figure~\ref{node_aggregation}). Rather than transmitting raw messages, it instead, forward residual error of the difference between the predicted representation and the aggregation  which reduce the dynamic range of the message being transmitted hence acting as low pass filter. Lastly, unlike the standard GNN that are trained using BP, where the update of weights corresponding to a given neighborhood are dependent, which create a large computation graphs, GPCN learning rules are local and the model weight are updated through energy minimization as we described in the methodology section.

\begin{figure}[H]
    \centering
    \includegraphics[width=3cm]{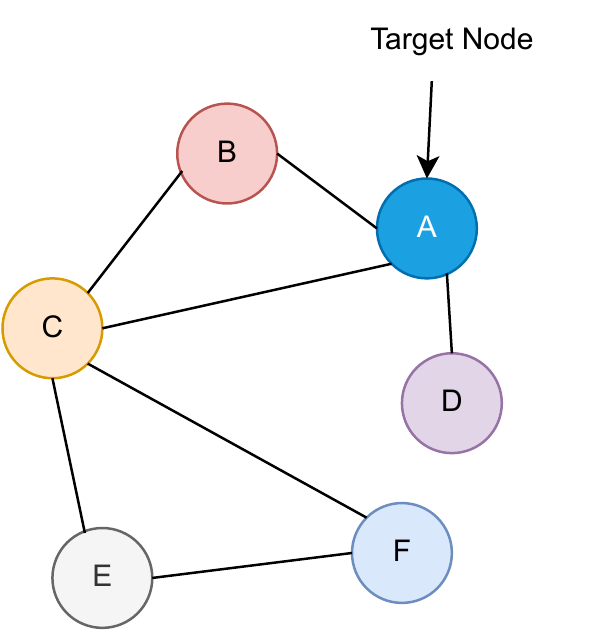}
    \caption{Example of graph that we use to illustrate the architecture.}
    \label{fig:example_graph}
\end{figure}

\begin{figure}[H]
    \centering
    \makebox[\textwidth]{
    \includegraphics[width=\textwidth]{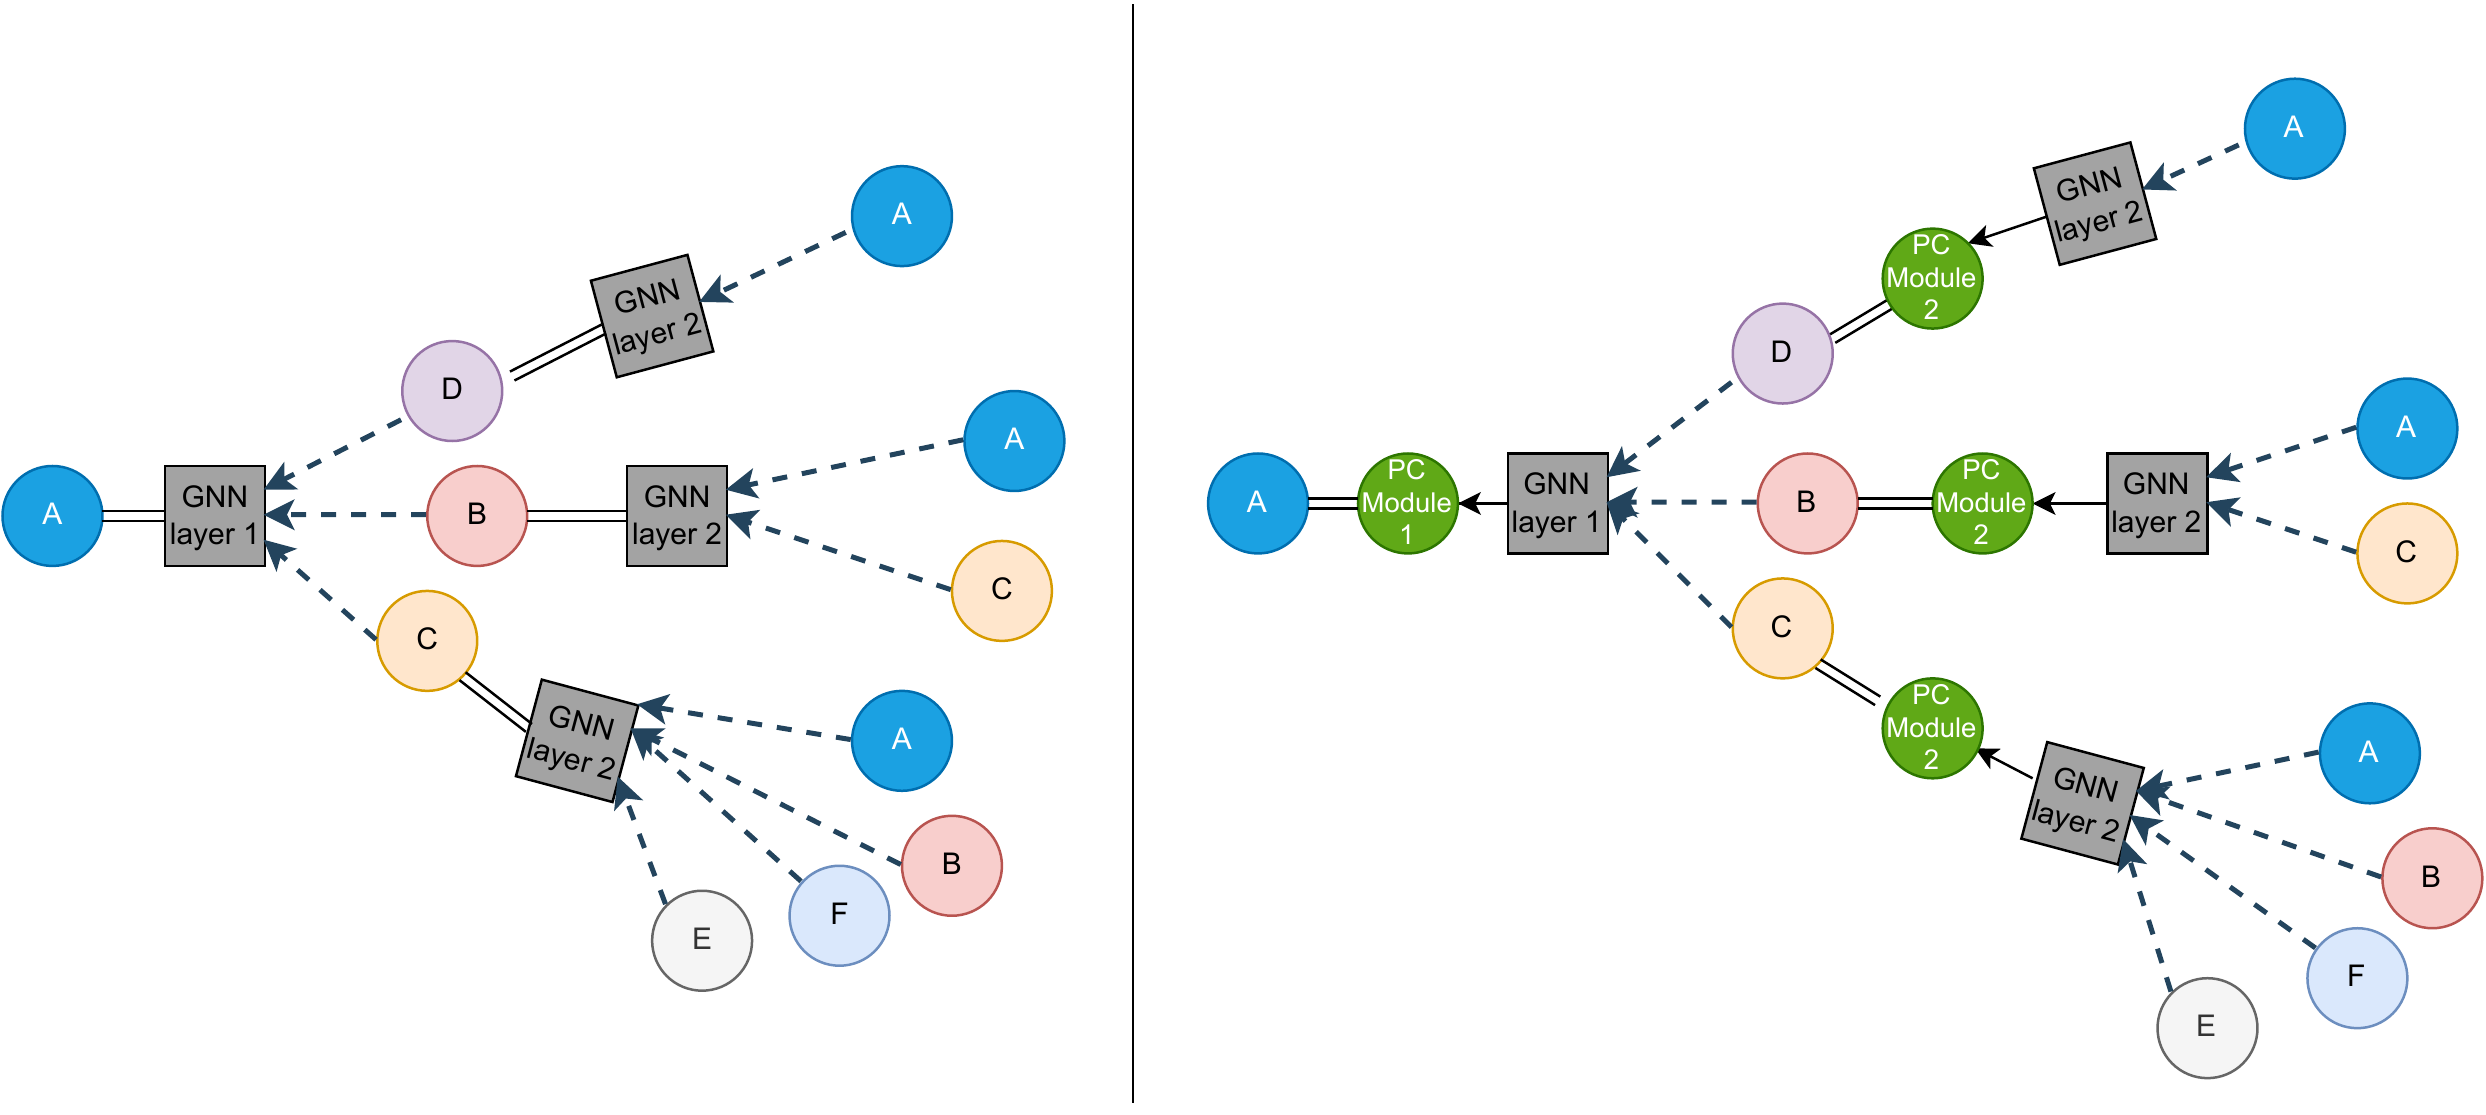}
    }
    \caption{Distinction of Messaging propagation between standard GNNs (Left) and inter-layer GPCN (Right).}
    \label{fig:graph_mesage_passing}
\end{figure}

\begin{figure}[H]
    \centering
    \makebox[\textwidth]{
    \includegraphics[width=\textwidth]{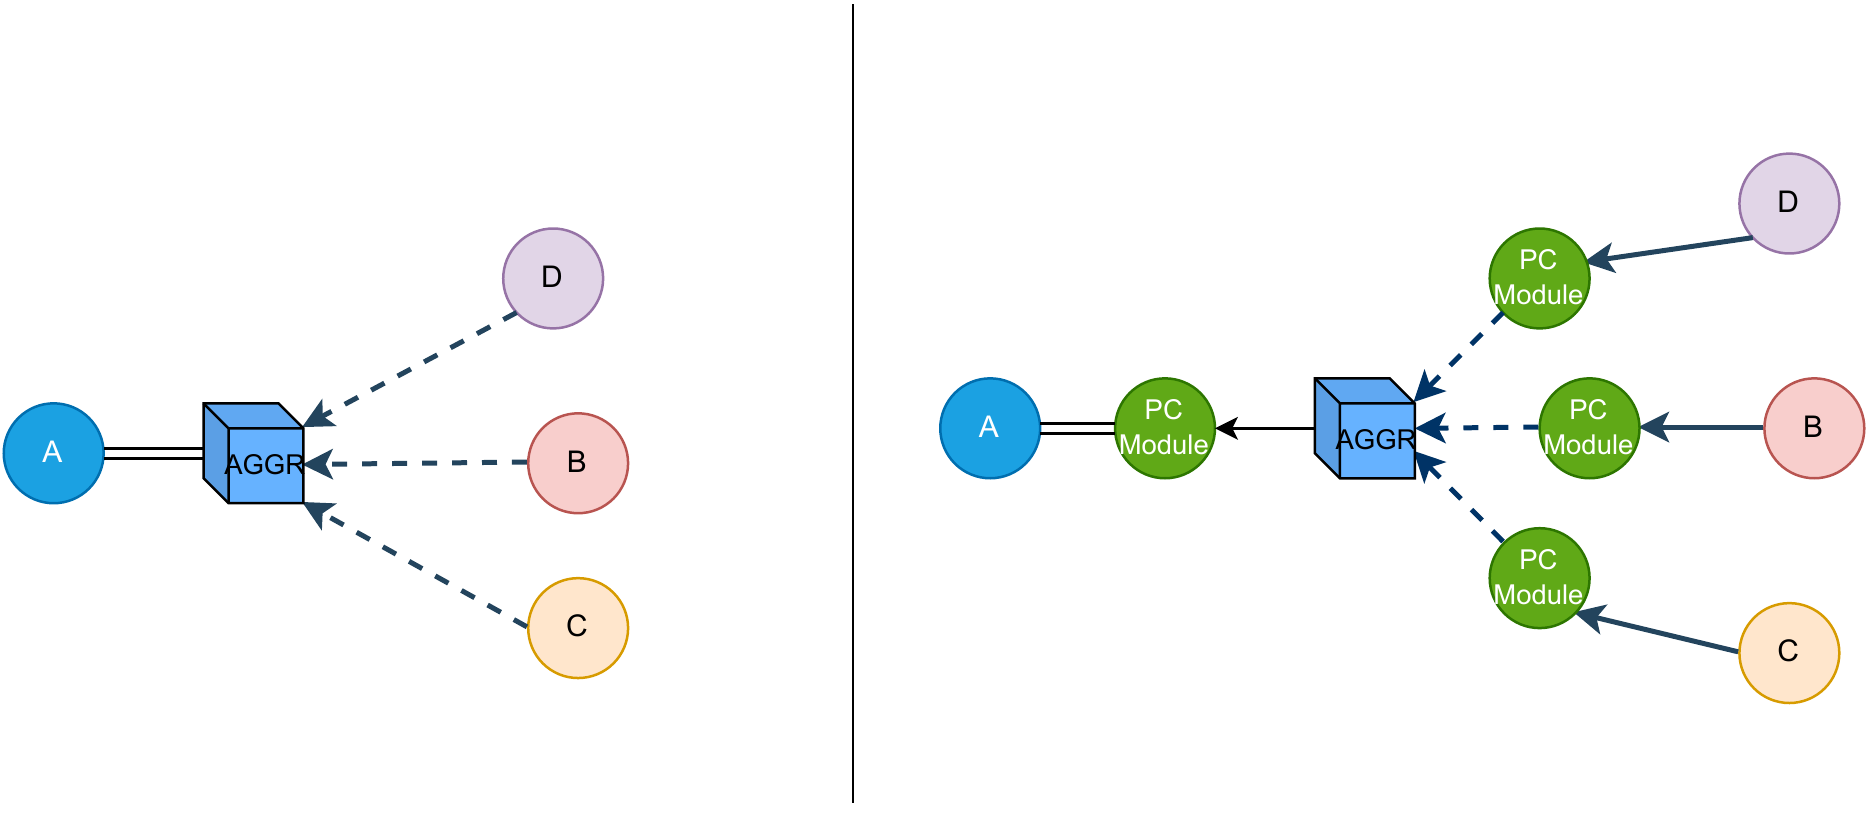}
    }
    \caption{Distinction of the difference between message aggregation between standard GNNs and GPCN. Left: standard aggregation method, Right: intra-layer GPCN.}
    \label{fig:node_aggregation}
\end{figure}

\section{Additional Results on Evasion Attacks with Nettack}

Due to the page constraint, here we provide additional results we could not include in the main body of this paper. In particular, the foloowing plots demonstrate how both GCN and GPCN model perform under various perturbation budgets on the four types of attacks namely feature, structure, feature-structure, and indirect attacks. 

\textbf{1) Structure and Feature attack:}

Figure~\ref{fig:both_s_f_attack1} show that with only 2 perturbation on neighbourhood structure and features of victim nodes, the median classification margin approaches -1 on GCN model, while GPCN stays relatively robust and with more robustness on lower energy model(PCx3) where most of the victims nodes have positive classification margins, or in other worlds, they are not adversarially affect by the attack. This trend is even pronounced when perturbation rate is increase to five(Figure~\ref{fig:both_s_f_attack2}) and ten (Figure~\ref{fig:both_s_f_attack3}) where, except for outliers, margin of classification of all victims nodes falls to $-1$ for both GCN and PC model PCx3 stay lately more robust.

\begin{figure}[H]
    \centering
    \makebox[\textwidth]{
    \includegraphics[width=\textwidth]{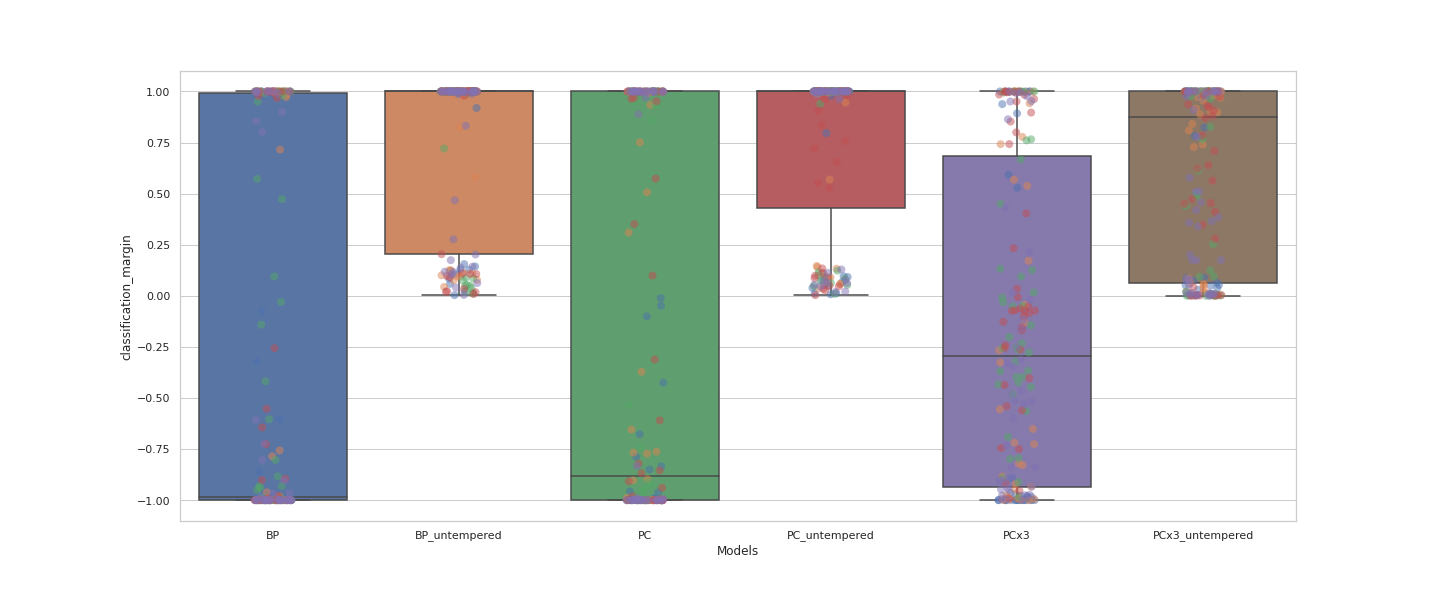}
    }
    \caption{Classification margin diagram of targeted attack on both features and structure when perturbation rate equal to 2. On x-axis BP indicates GCN model, PC denotes GPCN model trained of 12 inference steps, and  PCx3 indicate GPCN trained using 36 inference steps, hence achieves lower training energy. }
    \label{fig:both_s_f_attack1}
\end{figure}

\begin{figure}[H]
    \centering
    \makebox[\textwidth]{
    \includegraphics[width=\textwidth]{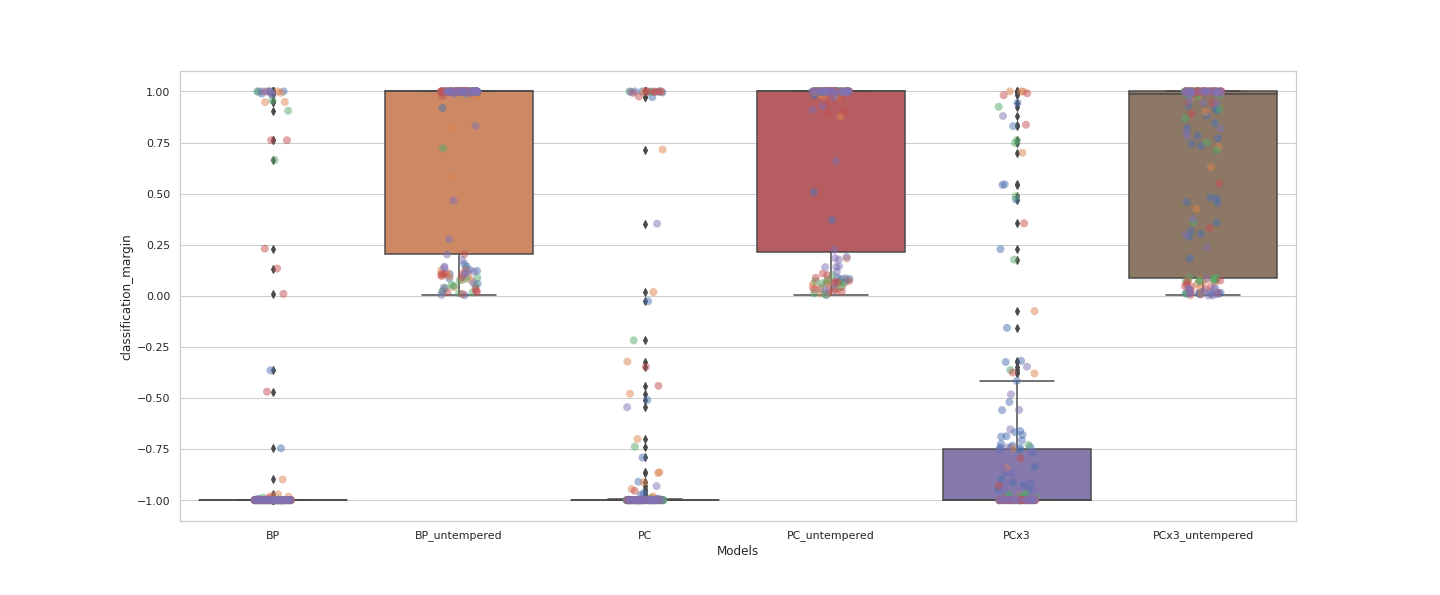}
    }
    \caption{Classification margin diagram of targeted attack on both features and structure when perturbation rate equal to 5}
    \label{fig:both_s_f_attack2}
\end{figure}

\begin{figure}[H]
    \centering
    \makebox[\textwidth]{
    \includegraphics[width=\textwidth]{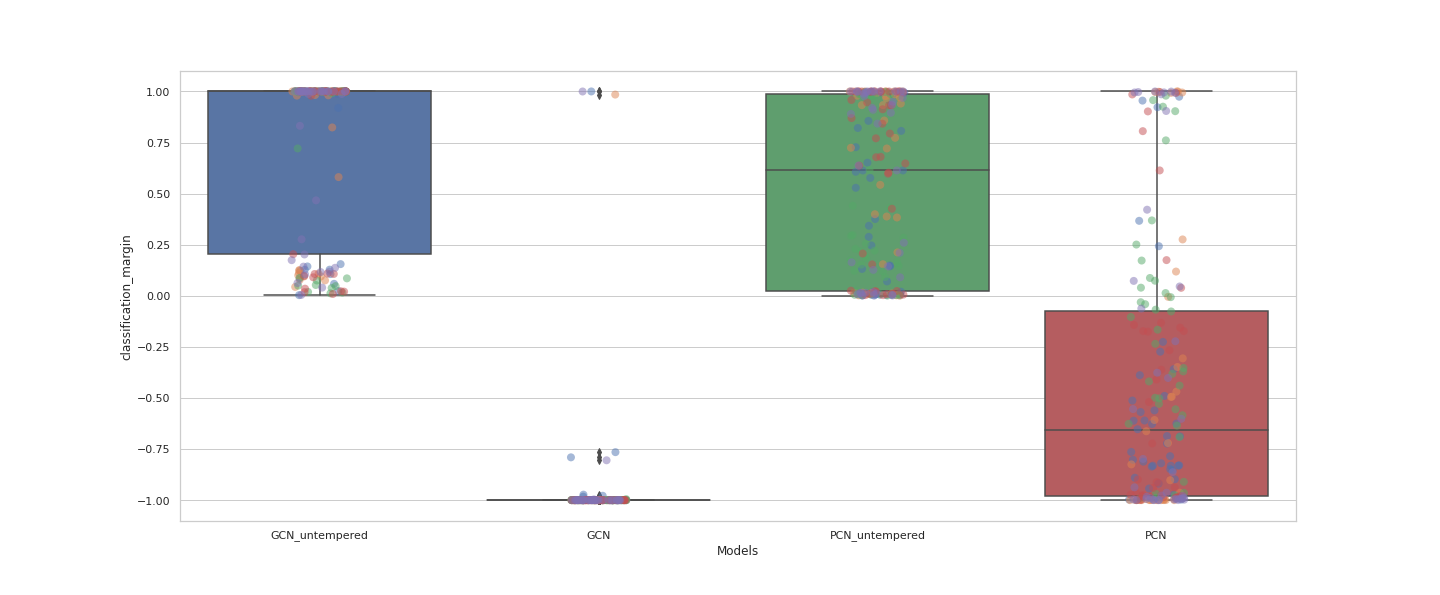}
    }
    \caption{Classification margin diagram of targeted attack on both features and structure when perturbation rate equal to 10}
    \label{fig:both_s_f_attack3}
\end{figure}

\textbf{2) Feature attacks}.
Since feature attacks do not high affect GNNs as much as structure attacks, we peform, large corruption of features with perturbation rate of 1, 5, 10, 30, 50 and 100. We observe a similar trends where with a small perturbation on features does not affect the model, however, when perturbation rate become large our GPCN display unparalleled performance resisting the attacks. When perturbation rate is equal to 30 (see Figure~\ref{fig:only_f_attack30}, while GCN misclassifies around $70\%$ of the victim nodes, GPCN is still able to classify more than $70\%$ correctly  after perturbation. The highly superior performance is observed when perturbation rate is increase to $100$ in Figure~\ref{fig:only_f_attack100}, GCN mislassifies all victims nodes, while GPCN still classify correctly those nodes with most victims nodes in the upper quartile having positive classification margins.

\begin{figure}[H]
    \centering
    \makebox[\textwidth]{
    \includegraphics[width=\textwidth]{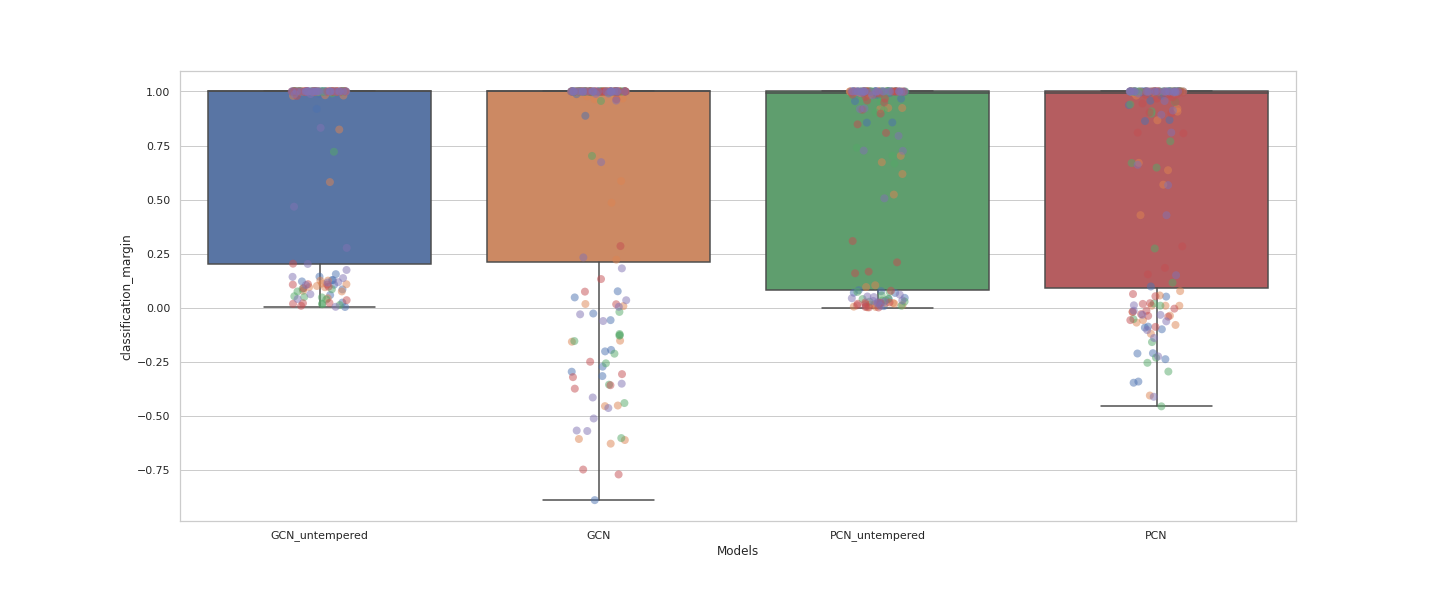}
    }
    \caption{Classification margin diagram of targeted attack on features when perturbation rate equal to 1}
    \label{fig:only_f_attack1}
\end{figure}

\begin{figure}[H]
    \centering
    \makebox[\textwidth]{
    \includegraphics[width=\textwidth]{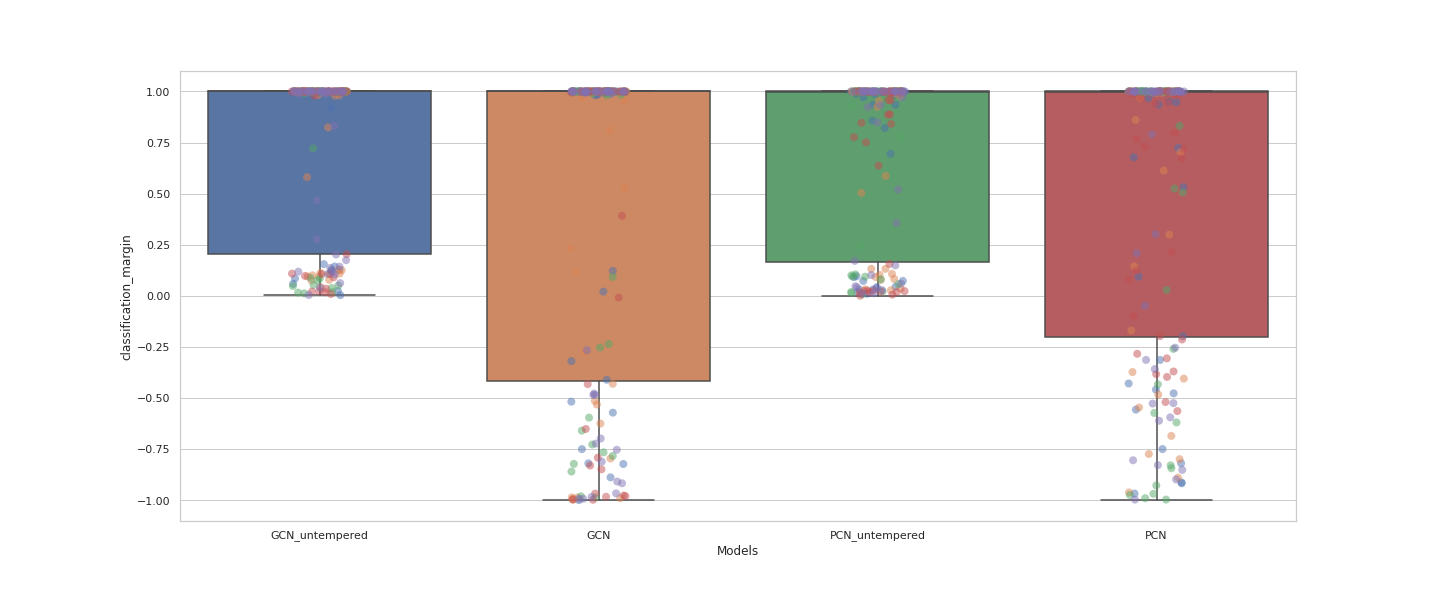}
    }
    \caption{Classification margin diagram of targeted attack on features when perturbation rate equal to 5}
    \label{fig:only_f_attack1}
\end{figure}

\begin{figure}[H]
    \centering
    \makebox[\textwidth]{
    \includegraphics[width=\textwidth]{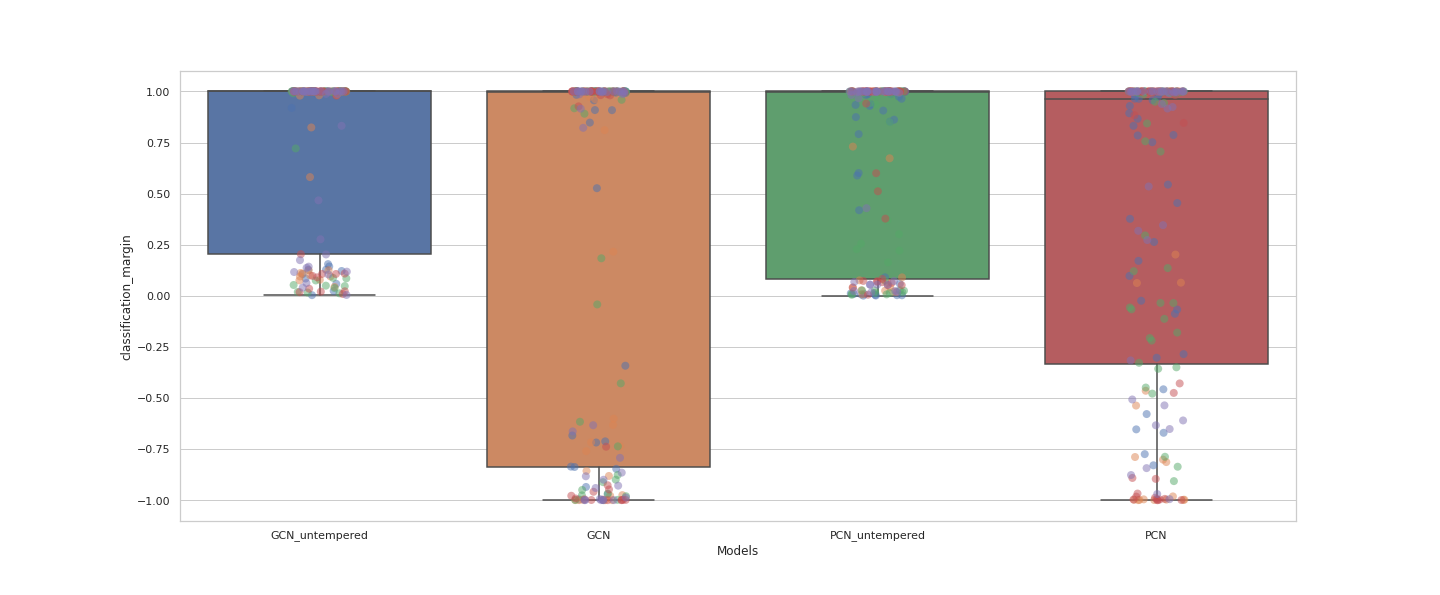}
    }
    \caption{Classification margin diagram of targeted attack on features when perturbation rate equal to 10}
    \label{fig:only_f_attack1}
\end{figure}

\begin{figure}[H]
    \centering
    \makebox[\textwidth]{
    \includegraphics[width=\textwidth]{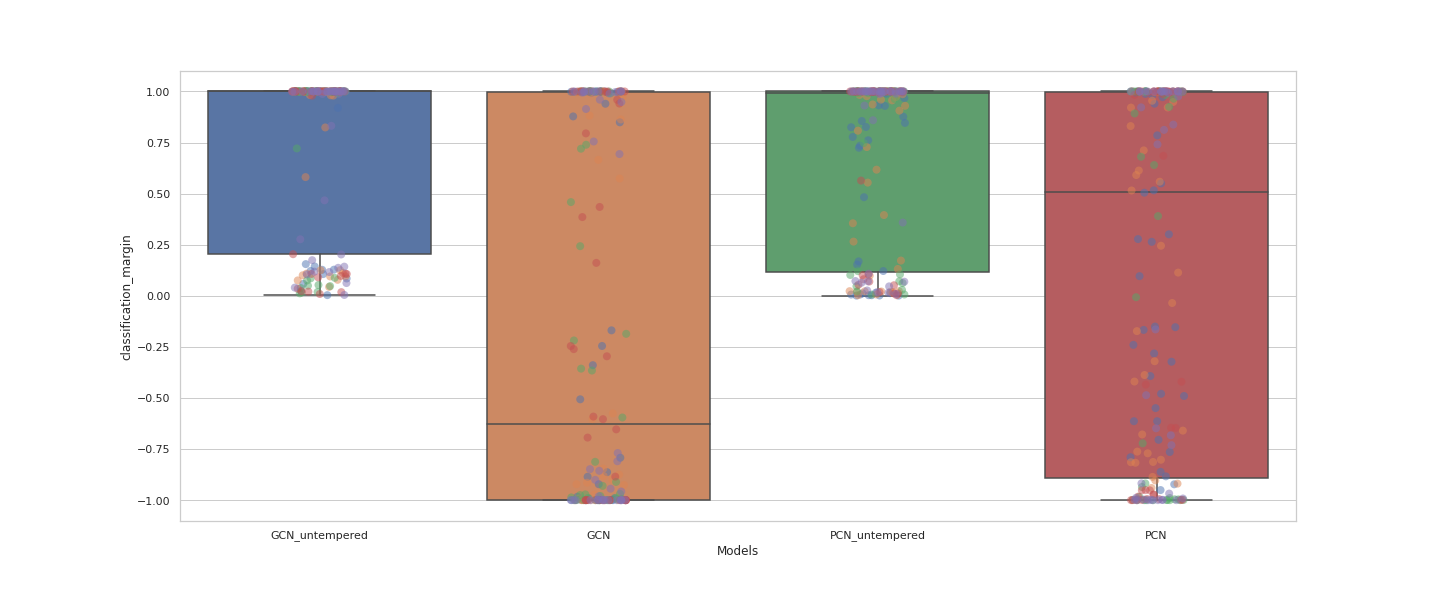}
    }
    \caption{Classification margin diagram of targeted attack on features when perturbation rate equal to 30}
    \label{fig:only_f_attack30}
\end{figure}

\begin{figure}[H]
    \centering
    \makebox[\textwidth]{
    \includegraphics[width=\textwidth]{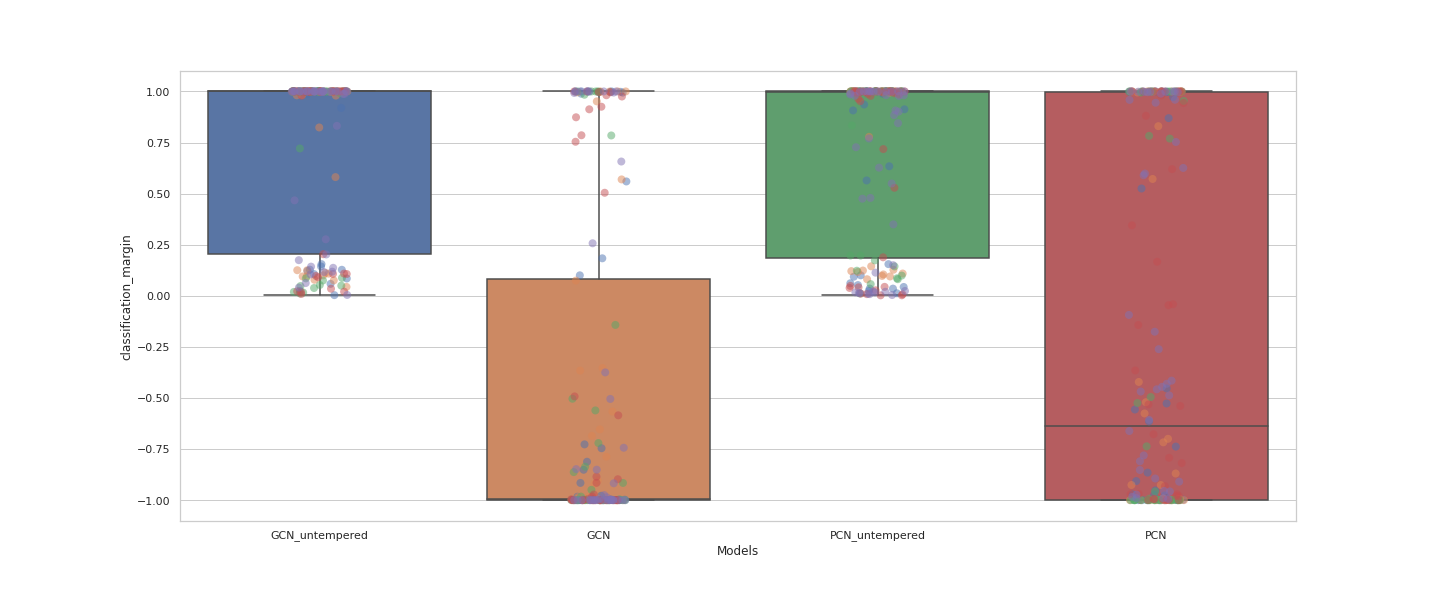}
    }
    \caption{Classification margin diagram of targeted attack on features when perturbation rate equal to 50}
    \label{fig:only_f_attack1}
\end{figure}

\begin{figure}[H]
    \centering
    \makebox[\textwidth]{
    \includegraphics[width=\textwidth]{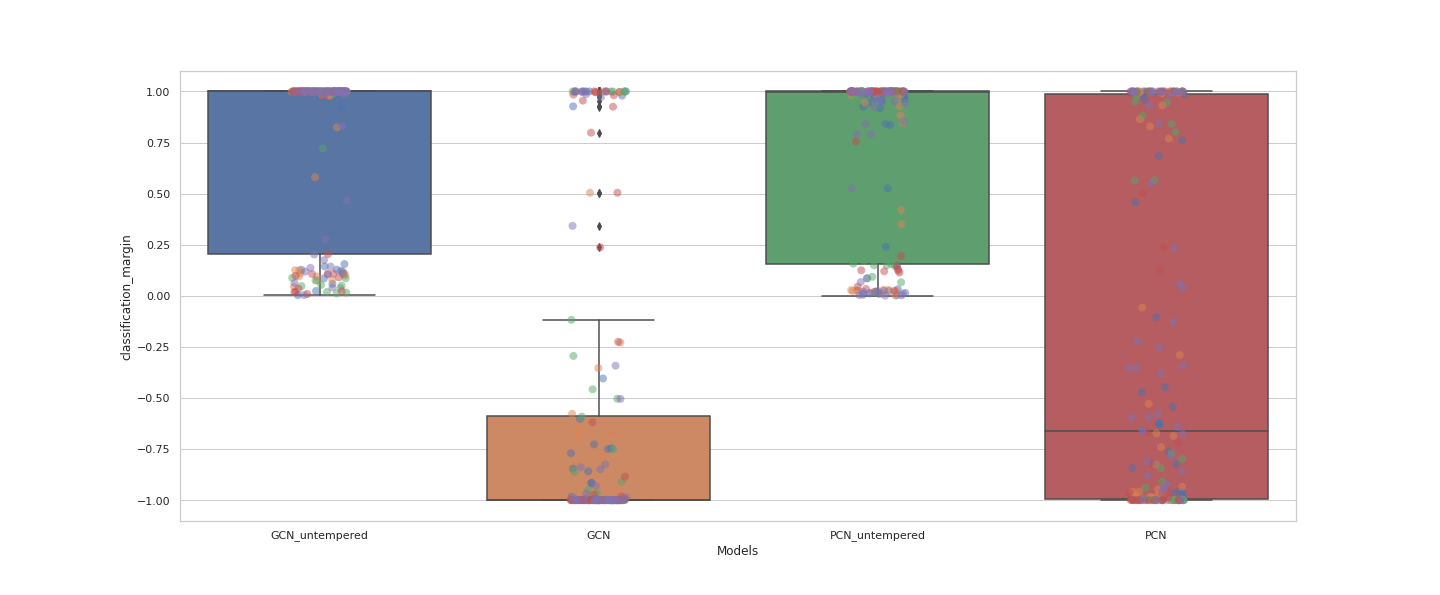}
    }
    \caption{Classification margin diagram of targeted attack on features when perturbation rate equal to 100}
    \label{fig:only_f_attack100}
\end{figure}

\textbf{3) Structure attacks}: GPCN also consistently outperforms GCN under structure-only attacks on number perturbation equal to 1, 2, 5 and 10 as it can be observed in Figure~\ref{fig:only_f_attack1},\ref{fig:only_f_attack2},\ref{fig:only_f_attack3},\ref{fig:only_f_attack5}, and \ref{fig:only_f_attack10}.

\begin{figure}[H]
    \centering
    \makebox[\textwidth]{
    \includegraphics[width=\textwidth]{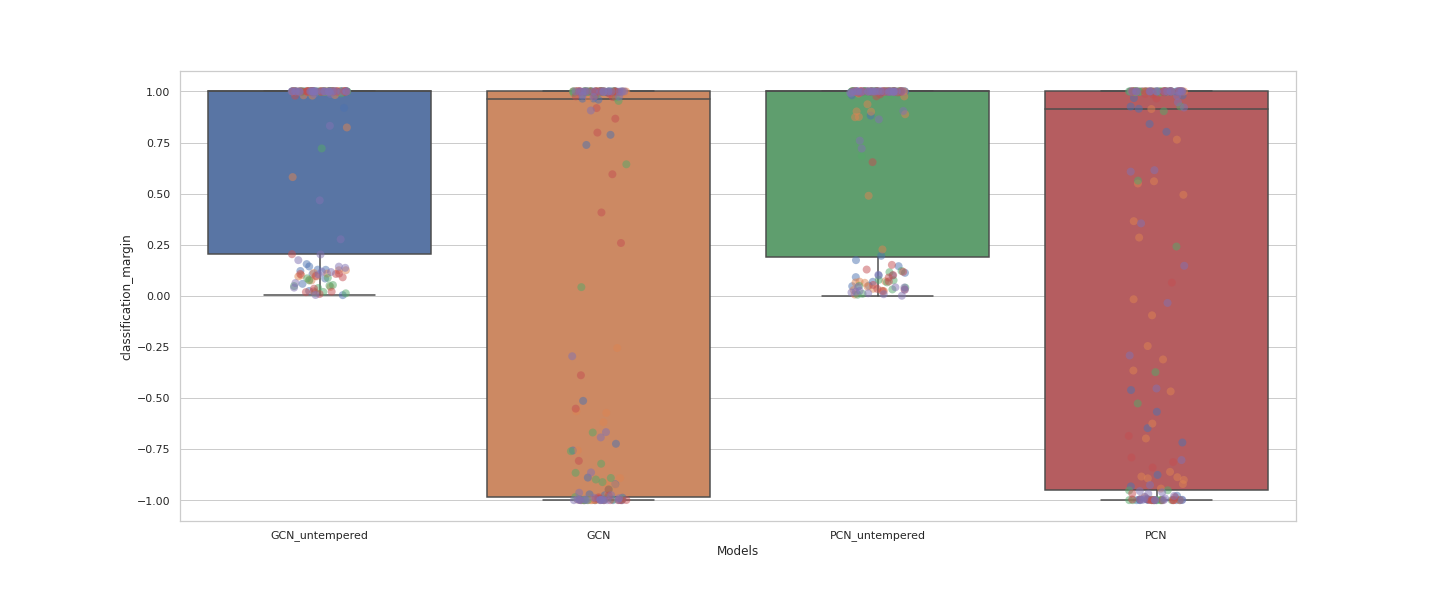}}
    \caption{Classification margin diagram of targeted attack on structure when perturbation rate equal to 1}
    \label{fig:only_f_attack1}
\end{figure}

\begin{figure}[H]
    \centering
    \makebox[\textwidth]{
    \includegraphics[width=\textwidth]{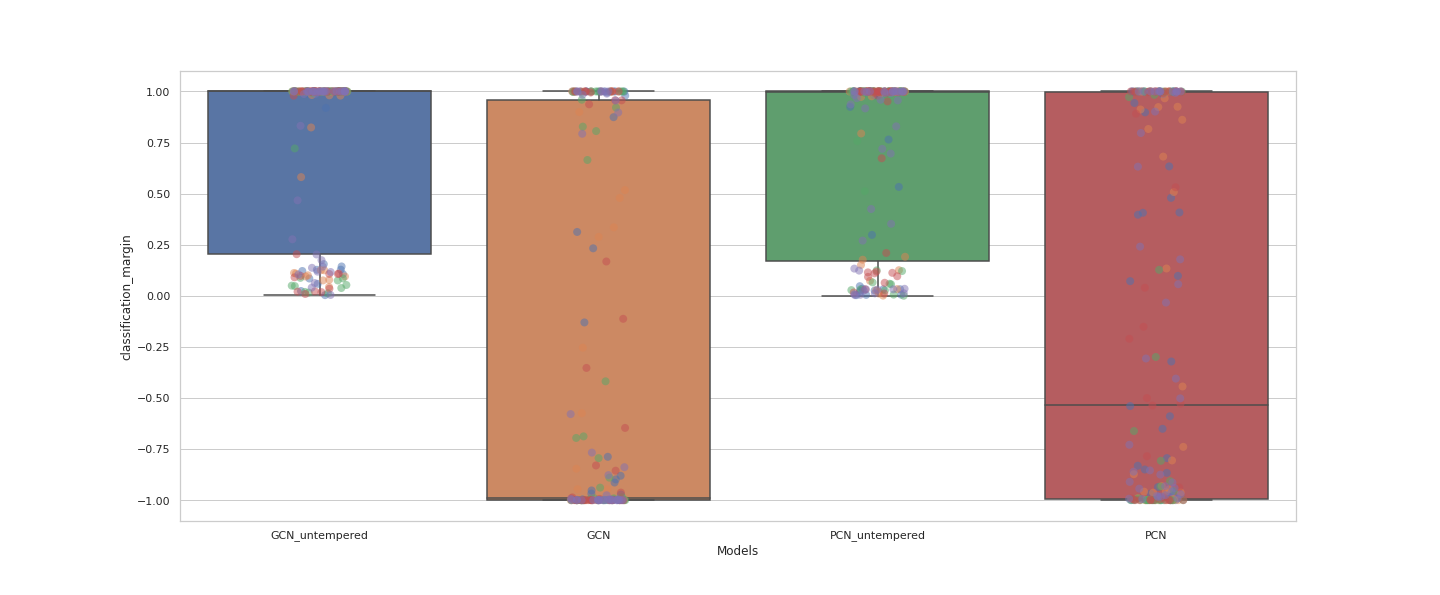}}
    \caption{Classification margin diagram of targeted attack on structure when perturbation rate equal to 2}
    \label{fig:only_f_attack2}
\end{figure}

\begin{figure}[H]
    \centering
    \makebox[\textwidth]{
    \includegraphics[width=\textwidth]{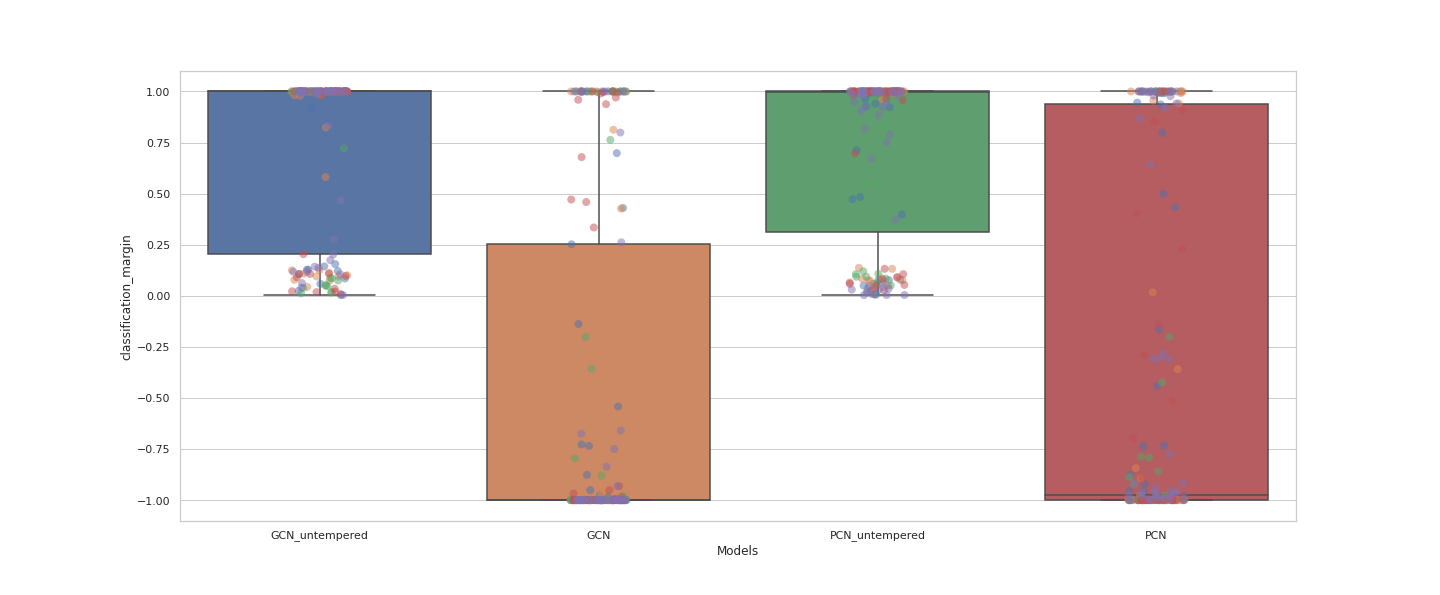}}
    \caption{Classification margin diagram of targeted attack on structure when perturbation rate equal to 3}
    \label{fig:only_f_attack3}
\end{figure}

\begin{figure}[H]
    \centering
    \makebox[\textwidth]{
    \includegraphics[width=\textwidth]{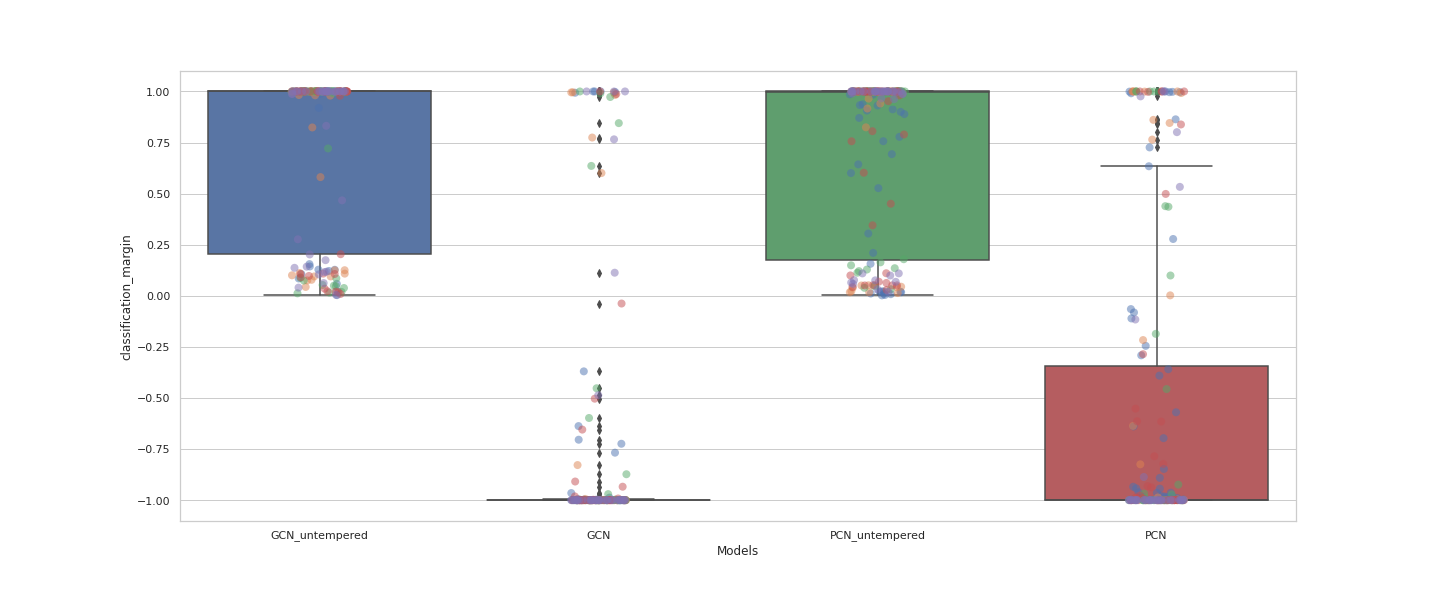}}
    \caption{Classification margin diagram of targeted attack on structure when perturbation rate equal to 5}
    \label{fig:only_f_attack5}
\end{figure}

\begin{figure}[H]
    \centering
    \makebox[\textwidth]{
    \includegraphics[width=\textwidth]{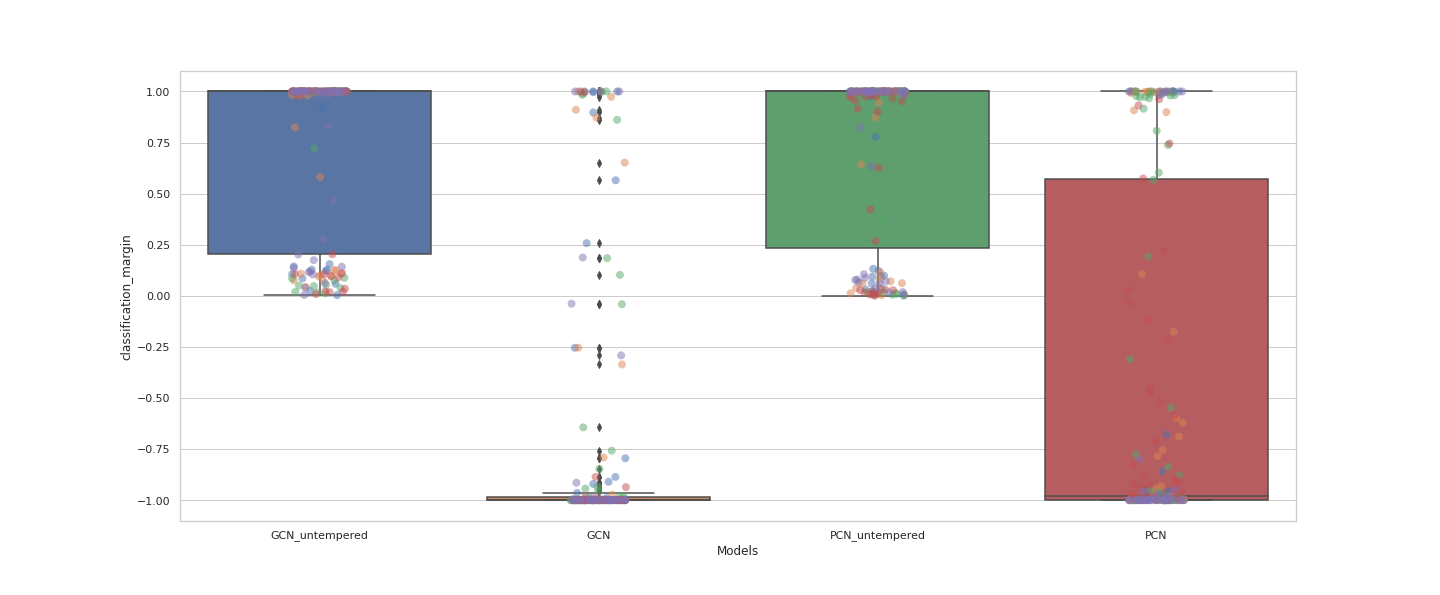}}
    \caption{Classification margin diagram of targeted attack on structure when perturbation rate equal to 10}
    \label{fig:only_f_attack10}
\end{figure}

\textbf{4) Indirect Attacks}:

For indirect attacks, we choose 5 influencing/neighboring nodes to attack for each victims node. We observe a similar trend that was found in the Nettack paper\cite{zugner2018adversarial}. We found that the influence or indirect attacks do not affects GNNs as much as other attacks as it can be witnessed from the box plots below. However, we also found that GPCN, especially one with smaller inference steps consistently outperforms all models, but all GPCN models are strictly better than GCN under all perturbations.

Note for Figure~\ref{fig:influence_attach_attack1}, \ref{fig:influence_attach_attack2}, and \ref{fig:influence_attach_attack3}, on x-axis, BP indicates GCN model, PC denotes GPCN model trained of 12 inference steps, and  PCx3 indicate GPCN trained using 36 inference steps, hence achieves lower training energy. The suffix 'untempered' indicates the performance of model on clean graph. To interpret the plots, a more robust model is one that retain a higher classification margins after the attacks.

\begin{figure}[H]
    \centering
    \makebox[\textwidth]{
    \includegraphics[width=\textwidth]{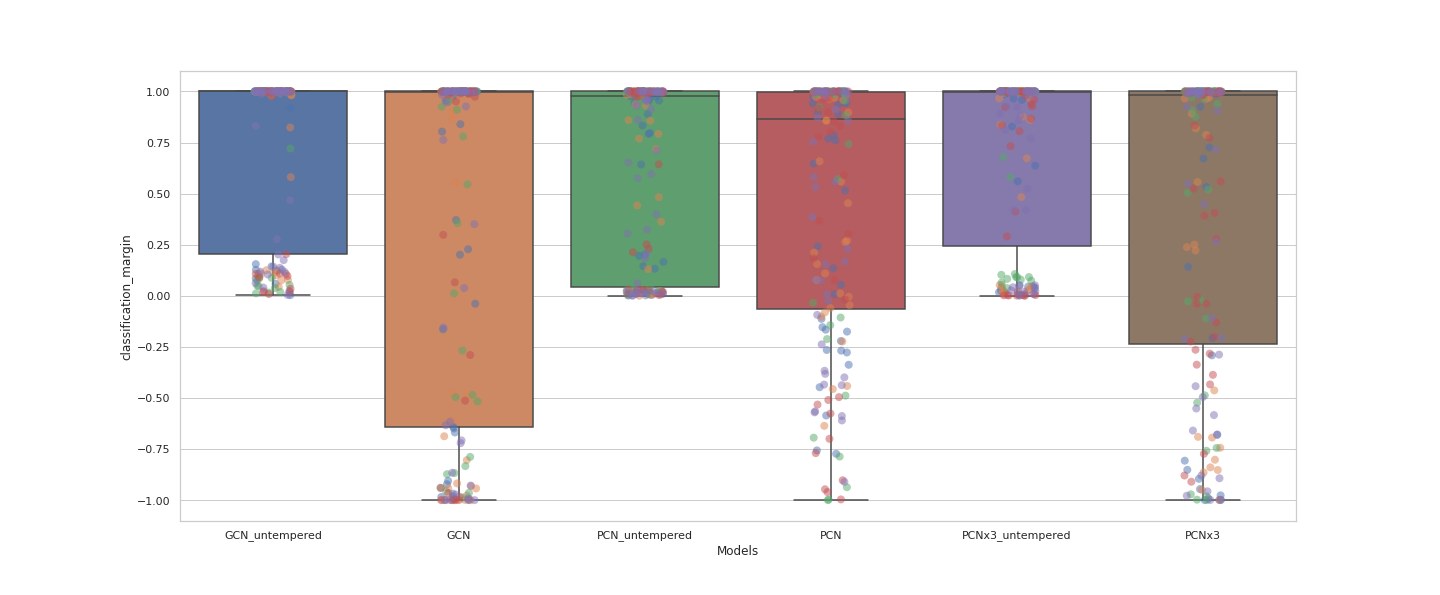}
    }
    \caption{Classification Margin Diagram on influence attack with perturbation equal to the degree of target node and 5 influencing neighboring nodes}
    \label{fig:influence_attach_attack1}
\end{figure}

\begin{figure}[H]
    \centering
    \makebox[\textwidth]{
    \includegraphics[width=\textwidth]{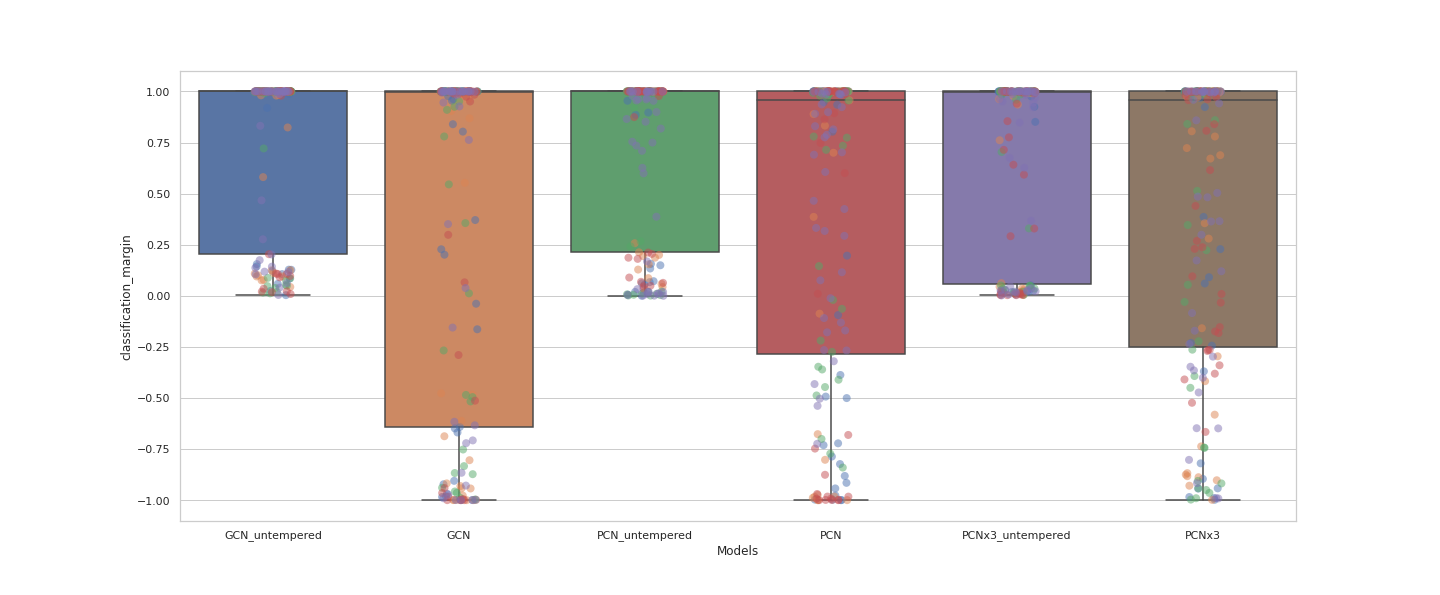}
    }
    \caption{Classification Margin Diagram on on influence attack with perturbation equal to the degree of target node and 5 influencing neighboring nodes}
    \label{fig:influence_attach_attack2}
\end{figure}

\begin{figure}[H]
    \centering
    \makebox[\textwidth]{
    \includegraphics[width=\textwidth]{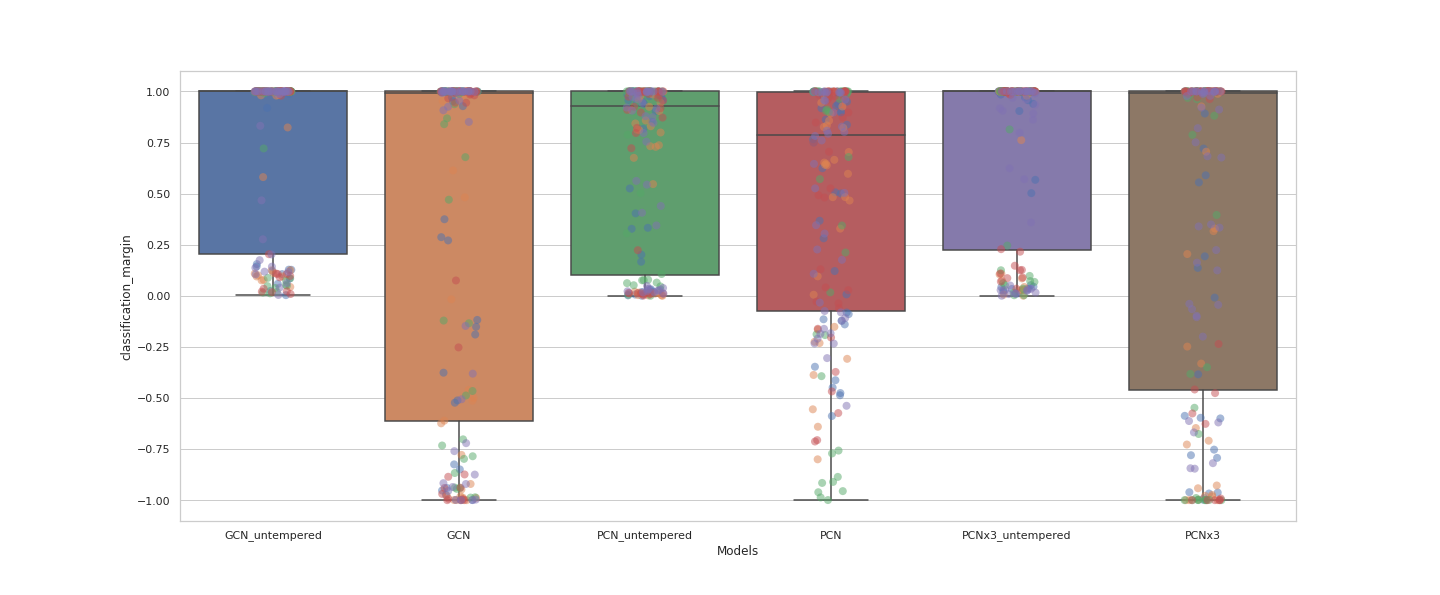}
    }
    \caption{Classification Margin Diagram on influence attack with perturbation equal to 1 and 5 influencing neighboring nodes}
    \label{fig:influence_attach_attack3}
\end{figure}

\begin{figure}[H]
    \centering
    \makebox[\textwidth]{
    \includegraphics[width=\textwidth]{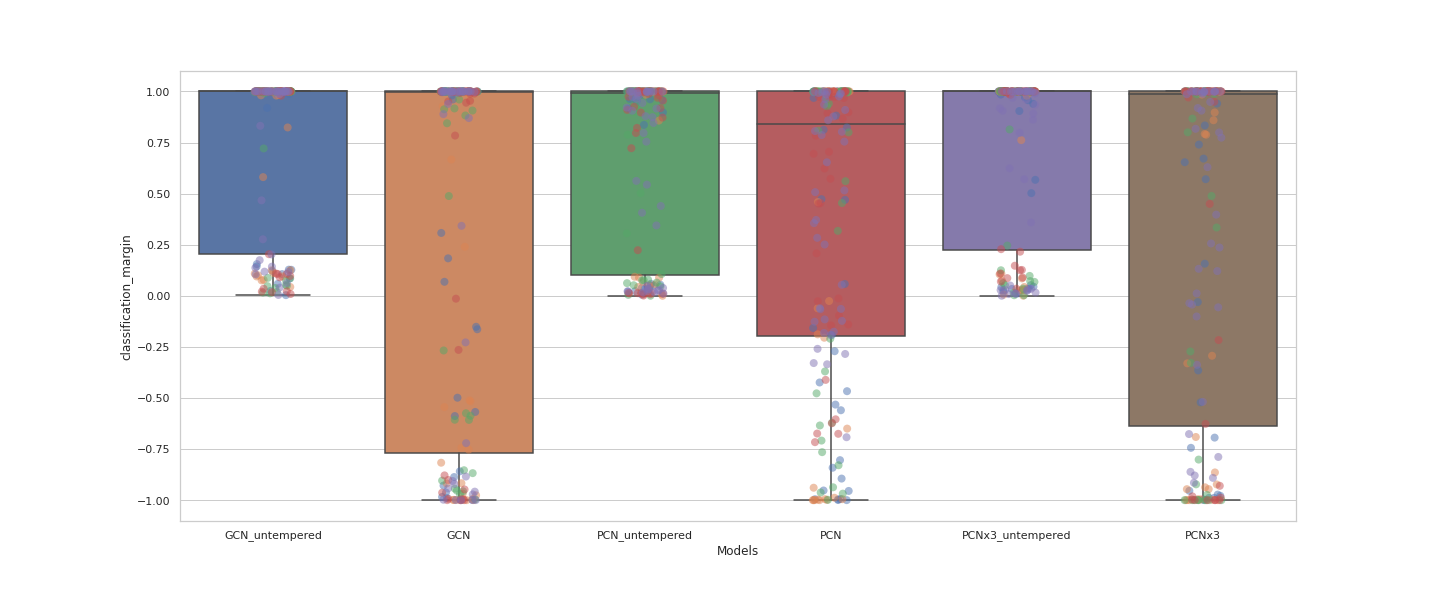}
    }
    \caption{Classification Margin Diagram on on influence attack with perturbation 10 and 5 influencing neighboring nodes}
    \label{fig:influence_attach_attack4}
\end{figure}
